# Supplementary material for: Alternant Hydrocarbon Diradicals as Optically Addressable Molecular Qubits
Source: arXiv:2403.09102 ancillary file (2024-03-18)
Supplement: Supplementary file 1 [file Supplementary_information.pdf]

Supplementary Information for

# Alternant Hydrocarbon Diradicals as Optically Addressable Molecular Qubits

Yong Rui Poh,[1] Dmitry Morozov,[2] Nathanael P. Kazmierczak,[3] Ryan G. Hadt,[3,*] Gerrit Groenhof,[4,*] and Joel Yuen-Zhou[1,*]

[1]Department of Chemistry and Biochemistry, University of California San Diego, La Jolla, California 92093, USA
[2]Terra Quantum AG, Kornhausstrasse 25, 9000 St. Gallen, Switzerland
[3]Division of Chemistry and Chemical Engineering, Arthur Amos Noyes Laboratory of Chemical Physics, California Institute of Technology, Pasadena, California 91125, USA
[4]Nanoscience Center and Department of Chemistry, University of Jyväskylä, Jyväskylä, Finland
*Corresponding authors. Email addresses: rghadt@caltech.edu (R.G.H.); gerrit.x.groenhof@jyu.fi (G.G.); joelyuen@ucsd.edu (J.Y.-Z.)

## Contents

**S1 Definitions of particle-hole transformation** 3

**S2 Expressions for the ground and lowest-lying excited electronic states** 3

**S3 Perturbation theory results** 7

**S4 Deriving the SOC operator for AHR $m$-dimers** 8

**S5 Results from configuration interaction between $\left|{}^3\mathbf{LE}_\Gamma^{10,+}; M_S\right\rangle$ and $\left|{}^3\mathbf{CT}_\Gamma^{10,+}; M_S\right\rangle$ states** 9

**S6 Deriving the energy expression for CS states** 10

**S7 Results from ab initio calculations of AHR $m$-dimers** 11

S7.1 Methylated benzylic radical $m$-dimer . . . 11

S7.1.1 DFT results . . . 11

S7.1.2 MCSCF/CI results . . . 15

S7.1.3 SOC matrix elements . . . 16

S7.2 TTM $m$-dimer . . . 19

S7.3 Removing two methyl substituents from the methylated benzylic radical $m$-dimer . . . 24

**S8 Results from ab initio calculations of AHRs** **24**

S8.1 Methylated benzylic radical . . . . . . . . . . . . . . . . . . . . . . . . . . . . . . . . 24

S8.2 TTM . . . . . . . . . . . . . . . . . . . . . . . . . . . . . . . . . . . . . . . . . . . . . . 27

## S1 Definitions of particle-hole transformation

We find Pariser's "+" and "−" labels [1, 2] to be identical to symmetries of an operator $\hat{P}_\mathrm{C}$ with the following action on "ordered" determinants $|\cdots\rangle_\mathrm{O}$:

$$\hat{P}_\mathrm{C}\left|\cdots(j+1)\,\overline{(j+1)}j\right\rangle_\mathrm{O} = -\left|\cdots 0\overline{0}\cdots(j-1)'\,\overline{(j-1)'}j'\right\rangle_\mathrm{O}, \tag{S1}$$

where "ordered" determinants are those written with increasing spin orbital indices[1]. As an example,

$$\hat{P}_\mathrm{C}\left|\Psi_{j}^{\overline{0}};+1/2\right\rangle = -\hat{P}_\mathrm{C}\left|\cdots j\cdots 0\overline{0}\right\rangle = \left|\cdots 1\overline{1}j'\right\rangle = \left|\Psi_{0}^{j'};+1/2\right\rangle, \tag{S2}$$

and indeed $\hat{P}_\mathrm{C}\left|\Psi_{0j}^{\pm};+1/2\right\rangle = \pm\left|\Psi_{0j}^{\pm};+1/2\right\rangle$. Meanwhile, the PHT $\hat{a}_{\mu\sigma}^\dagger \to f_\mu \hat{a}_{\mu\overline{\sigma}}$ is equivalent to $\hat{b}_{j_r\sigma}^\dagger \to \hat{b}_{j_r'\overline{\sigma}}$ in the MO basis because $c_{\mu j_r} = f_\mu c_{\mu j_r'}$ from the pairing theorem. Therefore, the two transformations achieve the same effect of converting occupied MOs into virtual ones. We note that the two definitions may sometimes return opposite symmetry labels; for instance, $\left|\Psi_{0j}^{+};+1/2\right\rangle$ is even ("+") in the first and odd in the second. However, because both definitions assign unique symmetries to each electronic state, they make the same predictions and are equivalent for our purposes, differing only in the notation.

## S2 Expressions for the ground and lowest-lying excited electronic states

Here, we list the expressions for the ground and lowest-lying singly-excited electronic states.

### Ground states

$$\left|{}^1\mathrm{GS};0\right\rangle \equiv \frac{1}{\sqrt{2}}\left(|\Psi;+1/2\rangle_A\otimes|\Psi;-1/2\rangle_B - |\Psi;-1/2\rangle_A\otimes|\Psi;+1/2\rangle_B\right), \tag{S3}$$

$$\left|{}^3\mathrm{GS};-1\right\rangle \equiv |\Psi;-1/2\rangle_A\otimes|\Psi;-1/2\rangle_B, \tag{S4}$$

$$\left|{}^3\mathrm{GS};0\right\rangle \equiv \frac{1}{\sqrt{2}}\left(|\Psi;+1/2\rangle_A\otimes|\Psi;-1/2\rangle_B + |\Psi;-1/2\rangle_A\otimes|\Psi;+1/2\rangle_B\right), \tag{S5}$$

$$\left|{}^3\mathrm{GS};+1\right\rangle \equiv |\Psi;+1/2\rangle_A\otimes|\Psi;+1/2\rangle_B, \tag{S6}$$

where subscripts label the monomer index $r \in \{A, B\}$ and $\left|\cdots j\overline{j}\right\rangle_A \otimes \left|\cdots k\overline{k}\right\rangle_B$ is to be interpreted as $\left|\cdots j_A\overline{j_A}\cdots k_B\overline{k_B}\right\rangle$.

### Local excitations

$S = 1, M_S = +1$:

$$\left|{}^3\mathrm{LE}_{\mathtt{A}}^{10,\pm};+1\right\rangle \equiv \frac{1}{\sqrt{2}}\left(\left|\Psi_{01}^{\pm};+1/2\right\rangle_A\otimes|\Psi;+1/2\rangle_B - |\Psi;+1/2\rangle_A\otimes\left|\Psi_{01}^{\pm};+1/2\right\rangle_B\right), \tag{S7}$$

$$\left|{}^3\mathrm{LE}_{\mathtt{B}}^{10,\pm};+1\right\rangle \equiv \frac{1}{\sqrt{2}}\left(\left|\Psi_{01}^{\pm};+1/2\right\rangle_A\otimes|\Psi;+1/2\rangle_B + |\Psi;+1/2\rangle_A\otimes\left|\Psi_{01}^{\pm};+1/2\right\rangle_B\right). \tag{S8}$$

[1] I.e. with ascending MO indices and, for doubly-occupied MOs, placing $\alpha$-spin before $\beta$-spin. For instance, $\left|\cdots\overline{1}0\overline{0}\right\rangle$ and $\left|\cdots 10\overline{0}\right\rangle$ are "ordered", but not $\left|\cdots 0\overline{1}\overline{0}\right\rangle$ and $\left|\cdots 1\overline{0}0\right\rangle$.

$S = 1, M_S = -1$:

$$\left|{}^3\mathrm{LE}^{10,\pm}_{\mathtt{A}}; -1\right\rangle \equiv \frac{1}{\sqrt{2}} \left( \left|\Psi^{\pm}_{01}; -1/2\right\rangle_A \otimes |\Psi; -1/2\rangle_B - |\Psi; -1/2\rangle_A \otimes \left|\Psi^{\pm}_{01}; -1/2\right\rangle_B \right), \tag{S9}$$

$$\left|{}^3\mathrm{LE}^{10,\pm}_{\mathtt{B}}; -1\right\rangle \equiv \frac{1}{\sqrt{2}} \left( \left|\Psi^{\pm}_{01}; -1/2\right\rangle_A \otimes |\Psi; -1/2\rangle_B + |\Psi; -1/2\rangle_A \otimes \left|\Psi^{\pm}_{01}; -1/2\right\rangle_B \right). \tag{S10}$$

$S = 1, M_S = 0$:

$$\left|{}^3\mathrm{LE}^{10,\pm}_{\mathtt{A}}; 0\right\rangle \equiv \frac{1}{\sqrt{2}} \left( \frac{\left|\Psi^{\pm}_{01}; +1/2\right\rangle_A \otimes |\Psi; -1/2\rangle_B + \left|\Psi^{\pm}_{01}; -1/2\right\rangle_A \otimes |\Psi; +1/2\rangle_B}{\sqrt{2}} - \frac{|\Psi; +1/2\rangle_A \otimes \left|\Psi^{\pm}_{01}; -1/2\right\rangle_B + |\Psi; -1/2\rangle_A \otimes \left|\Psi^{\pm}_{01}; +1/2\right\rangle_B}{\sqrt{2}} \right), \tag{S11}$$

$$\left|{}^3\mathrm{LE}^{10,\pm}_{\mathtt{B}}; 0\right\rangle \equiv \frac{1}{\sqrt{2}} \left( \frac{\left|\Psi^{\pm}_{01}; +1/2\right\rangle_A \otimes |\Psi; -1/2\rangle_B + \left|\Psi^{\pm}_{01}; -1/2\right\rangle_A \otimes |\Psi; +1/2\rangle_B}{\sqrt{2}} + \frac{|\Psi; +1/2\rangle_A \otimes \left|\Psi^{\pm}_{01}; -1/2\right\rangle_B + |\Psi; -1/2\rangle_A \otimes \left|\Psi^{\pm}_{01}; +1/2\right\rangle_B}{\sqrt{2}} \right). \tag{S12}$$

$S = 0, M_S = 0$:

$$\left|{}^1\mathrm{LE}^{10,\pm}_{\mathtt{A}}; 0\right\rangle \equiv \frac{1}{\sqrt{2}} \left( \frac{\left|\Psi^{\pm}_{01}; +1/2\right\rangle_A \otimes |\Psi; -1/2\rangle_B - \left|\Psi^{\pm}_{01}; -1/2\right\rangle_A \otimes |\Psi; +1/2\rangle_B}{\sqrt{2}} + \frac{|\Psi; +1/2\rangle_A \otimes \left|\Psi^{\pm}_{01}; -1/2\right\rangle_B - |\Psi; -1/2\rangle_A \otimes \left|\Psi^{\pm}_{01}; +1/2\right\rangle_B}{\sqrt{2}} \right), \tag{S13}$$

$$\left|{}^1\mathrm{LE}^{10,\pm}_{\mathtt{B}}; 0\right\rangle \equiv \frac{1}{\sqrt{2}} \left( \frac{\left|\Psi^{\pm}_{01}; +1/2\right\rangle_A \otimes |\Psi; -1/2\rangle_B - \left|\Psi^{\pm}_{01}; -1/2\right\rangle_A \otimes |\Psi; +1/2\rangle_B}{\sqrt{2}} - \frac{|\Psi; +1/2\rangle_A \otimes \left|\Psi^{\pm}_{01}; -1/2\right\rangle_B - |\Psi; -1/2\rangle_A \otimes \left|\Psi^{\pm}_{01}; +1/2\right\rangle_B}{\sqrt{2}} \right). \tag{S14}$$

## Charge transfer states

$S = 1, M_S = 1$:

$$\left|{}^3\mathrm{CT}^{10,\pm}_{\mathtt{A}}; +1\right\rangle \equiv \frac{1}{\sqrt{2}} \left( \left|{}^3\mathrm{CT}^{10}_{\mathtt{A}}; +1\right\rangle \pm \left|{}^3\mathrm{CT}^{01'}_{\mathtt{A}}; +1\right\rangle \right), \tag{S15}$$

$$\left|{}^3\mathrm{CT}^{10,\pm}_{\mathtt{B}}; +1\right\rangle \equiv \frac{1}{\sqrt{2}} \left( \left|{}^3\mathrm{CT}^{10}_{\mathtt{B}}; +1\right\rangle \mp \left|{}^3\mathrm{CT}^{01'}_{\mathtt{B}}; +1\right\rangle \right), \tag{S16}$$

where

$$\left|{}^3\mathrm{CT}^{10}_{\mathtt{A}}; +1\right\rangle \equiv \frac{1}{\sqrt{2}} \left( \left|{}^3\mathrm{GS}^{\overline{0_B}}_{\overline{1_A}}; +1\right\rangle - \left|{}^3\mathrm{GS}^{\overline{0_A}}_{\overline{1_B}}; +1\right\rangle \right), \tag{S17}$$

$$\left|{}^3\mathrm{CT}^{10}_{\mathtt{B}}; +1\right\rangle \equiv \frac{1}{\sqrt{2}} \left( \left|{}^3\mathrm{GS}^{\overline{0_B}}_{\overline{1_A}}; +1\right\rangle + \left|{}^3\mathrm{GS}^{\overline{0_A}}_{\overline{1_B}}; +1\right\rangle \right), \tag{S18}$$

$$\left|{}^3\mathrm{CT}^{01'}_{\mathtt{A}}; +1\right\rangle \equiv \frac{1}{\sqrt{2}} \left( \left|{}^3\mathrm{GS}^{1'_B}_{0_A}; +1\right\rangle - \left|{}^3\mathrm{GS}^{1'_A}_{0_B}; +1\right\rangle \right), \tag{S19}$$

$$\left|{}^3\mathrm{CT}^{01'}_{\mathtt{B}}; +1\right\rangle \equiv \frac{1}{\sqrt{2}} \left( \left|{}^3\mathrm{GS}^{1'_B}_{0_A}; +1\right\rangle + \left|{}^3\mathrm{GS}^{1'_A}_{0_B}; +1\right\rangle \right). \tag{S20}$$

$S = 1, M_S = -1$:

$$\left|{}^3\mathrm{CT}^{10,\pm}_{\mathtt{A}}; -1\right\rangle \equiv \frac{1}{\sqrt{2}} \left( \left|{}^3\mathrm{CT}^{10}_{\mathtt{A}}; -1\right\rangle \pm \left|{}^3\mathrm{CT}^{01'}_{\mathtt{A}}; -1\right\rangle \right), \tag{S21}$$

$$\left|{}^3\mathrm{CT}^{10,\pm}_{\mathtt{B}}; -1\right\rangle \equiv \frac{1}{\sqrt{2}} \left( \left|{}^3\mathrm{CT}^{10}_{\mathtt{B}}; -1\right\rangle \mp \left|{}^3\mathrm{CT}^{01'}_{\mathtt{B}}; -1\right\rangle \right), \tag{S22}$$

where

$$\left|{}^3\mathrm{CT}^{10}_{\mathtt{A}}; -1\right\rangle \equiv \frac{1}{\sqrt{2}} \left( \left|{}^3\mathrm{GS}^{0_B}_{1_A}; -1\right\rangle - \left|{}^3\mathrm{GS}^{0_A}_{1_B}; -1\right\rangle \right), \tag{S23}$$

$$\left|{}^3\mathrm{CT}^{10}_{\mathtt{B}}; -1\right\rangle \equiv \frac{1}{\sqrt{2}} \left( \left|{}^3\mathrm{GS}^{0_B}_{1_A}; -1\right\rangle + \left|{}^3\mathrm{GS}^{0_A}_{1_B}; -1\right\rangle \right), \tag{S24}$$

$$\left|{}^3\mathrm{CT}^{01'}_{\mathtt{A}}; -1\right\rangle \equiv \frac{1}{\sqrt{2}} \left( \left|{}^3\mathrm{GS}^{\overline{1'_B}}_{\overline{0_A}}; -1\right\rangle - \left|{}^3\mathrm{GS}^{\overline{1'_A}}_{\overline{0_B}}; -1\right\rangle \right), \tag{S25}$$

$$\left|{}^3\mathrm{CT}^{01'}_{\mathtt{B}}; -1\right\rangle \equiv \frac{1}{\sqrt{2}} \left( \left|{}^3\mathrm{GS}^{\overline{1'_B}}_{\overline{0_A}}; -1\right\rangle + \left|{}^3\mathrm{GS}^{\overline{1'_A}}_{\overline{0_B}}; -1\right\rangle \right). \tag{S26}$$

$S = 1, M_S = 0$:

$$\left|{}^3\mathrm{CT}^{10,\pm}_{\mathtt{A}}; 0\right\rangle \equiv \frac{1}{\sqrt{2}} \left( \left|{}^3\mathrm{CT}^{10}_{\mathtt{A}}; 0\right\rangle \pm \left|{}^3\mathrm{CT}^{01'}_{\mathtt{A}}; 0\right\rangle \right), \tag{S27}$$

$$\left|{}^3\mathrm{CT}^{10,\pm}_{\mathtt{B}}; 0\right\rangle \equiv \frac{1}{\sqrt{2}} \left( \left|{}^3\mathrm{CT}^{10}_{\mathtt{B}}; 0\right\rangle \mp \left|{}^3\mathrm{CT}^{01'}_{\mathtt{B}}; 0\right\rangle \right), \tag{S28}$$

where

$$\left|{}^3\mathrm{CT}^{10}_{\mathtt{A}}; 0\right\rangle \equiv \frac{1}{\sqrt{2}} \left( \left|{}^3\mathrm{GS}^{0_B}_{1_A}; 0\right\rangle - \left|{}^3\mathrm{GS}^{\overline{0_A}}_{\overline{1_B}}; 0\right\rangle \right), \tag{S29}$$

$$\left|{}^3\mathrm{CT}^{10}_{\mathtt{B}}; 0\right\rangle \equiv \frac{1}{\sqrt{2}} \left( \left|{}^3\mathrm{GS}^{0_B}_{1_A}; 0\right\rangle + \left|{}^3\mathrm{GS}^{\overline{0_A}}_{\overline{1_B}}; 0\right\rangle \right), \tag{S30}$$

$$\left|{}^3\mathrm{CT}^{01'}_{\mathtt{A}}; 0\right\rangle \equiv \frac{1}{\sqrt{2}} \left( \left|{}^3\mathrm{GS}^{1'_B}_{0_A}; 0\right\rangle - \left|{}^3\mathrm{GS}^{\overline{1'_A}}_{\overline{0_B}}; 0\right\rangle \right), \tag{S31}$$

$$\left|{}^3\mathrm{CT}^{01'}_{\mathtt{B}}; 0\right\rangle \equiv \frac{1}{\sqrt{2}} \left( \left|{}^3\mathrm{GS}^{1'_B}_{0_A}; 0\right\rangle + \left|{}^3\mathrm{GS}^{\overline{1'_A}}_{\overline{0_B}}; 0\right\rangle \right), \tag{S32}$$

and $\left|{}^3\mathrm{GS}^{0_B}_{1_A}; 0\right\rangle$ is to be interpreted as $1_A \to 0_B$ of the first term and $\overline{1_A} \to \overline{0_B}$ of the second term in $\left|{}^3\mathrm{GS}; 0\right\rangle$, i.e. the label corresponds to the excitation of the first term in $\left|{}^3\mathrm{GS}; 0\right\rangle$.

$S = 0, M_S = 0$:

$$\left|{}^1\mathrm{CT}^{10,\pm}_{\mathtt{A}}; 0\right\rangle \equiv \frac{1}{\sqrt{2}} \left( \left|{}^1\mathrm{CT}^{10}_{\mathtt{A}}; 0\right\rangle \mp \left|{}^1\mathrm{CT}^{01'}_{\mathtt{A}}; 0\right\rangle \right), \tag{S33}$$

$$\left|{}^1\mathrm{CT}^{10,\pm}_{\mathtt{B}}; 0\right\rangle \equiv \frac{1}{\sqrt{2}} \left( \left|{}^1\mathrm{CT}^{10}_{\mathtt{B}}; 0\right\rangle \pm \left|{}^1\mathrm{CT}^{01'}_{\mathtt{B}}; 0\right\rangle \right), \tag{S34}$$

$$\left|{}^1\mathrm{CT}^{00,-}_{\mathtt{A}}; 0\right\rangle \equiv \frac{1}{\sqrt{2}} \left( \left|{}^1\mathrm{GS}^{0_B}_{0_A}; 0\right\rangle + \left|{}^1\mathrm{GS}^{\overline{0_A}}_{\overline{0_B}}; 0\right\rangle \right), \tag{S35}$$

$$\left|{}^1\mathrm{CT}^{00,+}_{\mathtt{B}}; 0\right\rangle \equiv \frac{1}{\sqrt{2}} \left( \left|{}^1\mathrm{GS}^{0_B}_{0_A}; 0\right\rangle - \left|{}^1\mathrm{GS}^{\overline{0_A}}_{\overline{0_B}}; 0\right\rangle \right), \tag{S36}$$

where

$$\left|{}^{1}\mathrm{CT}^{10}_{\mathtt{A}};0\right\rangle \equiv \frac{1}{\sqrt{2}}\left(\left|{}^{1}\mathrm{GS}^{0_B}_{1_A};0\right\rangle + \left|{}^{1}\mathrm{GS}^{\overline{0_A}}_{\overline{1_B}};0\right\rangle\right), \tag{S37}$$

$$\left|{}^{1}\mathrm{CT}^{10}_{\mathtt{B}};0\right\rangle \equiv \frac{1}{\sqrt{2}}\left(\left|{}^{1}\mathrm{GS}^{0_B}_{1_A};0\right\rangle - \left|{}^{1}\mathrm{GS}^{\overline{0_A}}_{\overline{1_B}};0\right\rangle\right), \tag{S38}$$

$$\left|{}^{1}\mathrm{CT}^{01'}_{\mathtt{A}};0\right\rangle \equiv \frac{1}{\sqrt{2}}\left(\left|{}^{1}\mathrm{GS}^{1'_B}_{0_A};0\right\rangle + \left|{}^{1}\mathrm{GS}^{\overline{1'_A}}_{\overline{0_B}};0\right\rangle\right), \tag{S39}$$

$$\left|{}^{1}\mathrm{CT}^{01'}_{\mathtt{B}};0\right\rangle \equiv \frac{1}{\sqrt{2}}\left(\left|{}^{1}\mathrm{GS}^{1'_B}_{0_A};0\right\rangle - \left|{}^{1}\mathrm{GS}^{\overline{1'_A}}_{\overline{0_B}};0\right\rangle\right), \tag{S40}$$

and $\left|{}^{1}\mathrm{GS}^{0_B}_{1_A};0\right\rangle$ is to be interpreted as $1_A \to 0_B$ of the first term and $\overline{1_A} \to \overline{0_B}$ of the second term in $\left|{}^{1}\mathrm{GS};0\right\rangle$, i.e. the label corresponds to the excitation of the first term in $\left|{}^{1}\mathrm{GS};0\right\rangle$.

# S3 Perturbation theory results

**Table S1**: Properties of ground and low-lying excited electronic states of AHR $m$-dimers, presented approximately in increasing order of zeroth-order energies. Definitions: $\varepsilon_j$ = energy of monoradical's $j$-th MO; $J_{jk} = (jj|kk)$ and $K_{jk} = (jk|kj)$ in chemists' notation [3]; $c_{\mathcal{A}1} = (c_{\mathcal{B}1} =)$ coefficient of the AO at the dimer linkage to the HOMO–1 of monomer $A$ $(B)$, assumed to be real-valued; $\{|\Phi_j\rangle\,|j\}$ = set containing states $|\Phi_j\rangle$ of all possible values $j$.

| State | Energy | Corrected state to $\mathcal{O}(V_{\mathbf{NN}})$ | Corrected energy to $\mathcal{O}(V_{\mathbf{NN}}^2)$ | Transition dipole moment |
|---|---|---|---|---|
| $\{\lvert^{2S+1}\mathrm{GS};M_S\rangle\,\lvert S,M_S\}$ | $0$ | $\{\lvert^{2S+1}\mathrm{GS};M_S\rangle\,\lvert S,M_S\}$ | $\gamma_{\mathcal{AB}}$ | – |
| $\lvert^{1}\mathrm{CT}^{00,-}_{\mathtt{A}};0\rangle;\lvert^{1}\mathrm{CT}^{00,+}_{\mathtt{B}};0\rangle$ | $J_{00}$ | $\lvert^{1}\mathrm{CT}^{00,-}_{\mathtt{A}};0\rangle;\lvert^{1}\mathrm{CT}^{00,+}_{\mathtt{B}};0\rangle$ | $J_{00}+\gamma_{\mathcal{AB}}$ | 0 |
| $\{\lvert^{2S+1}\mathrm{LE}^{10,-}_{\Gamma};M_S\rangle\,\lvert S,M_S,\Gamma\}$ | $E(\mathrm{LE}^-)\equiv(\varepsilon_0-\varepsilon_1)$ | $\{\lvert^{3}\mathrm{LE}^{10,-}_{\mathtt{A}};M_S\rangle+\frac{c_{\mathcal{A}1}c_{\mathcal{B}1}\beta_{\mathcal{AB}}}{J_{10}}\lvert^{3}\mathrm{CT}^{10,-}_{\mathtt{A}};M_S\rangle\}$ | $(1+c_{\mathcal{A}1}c_{\mathcal{A}1})\gamma_{\mathcal{AB}}$ | 0 |
| | $-J_{10}+\frac{1}{2}J_{00}-\frac{1}{2}K_{10}$ | $\{\lvert^{3}\mathrm{LE}^{10,-}_{\mathtt{B}};M_S\rangle-\frac{c_{\mathcal{A}1}c_{\mathcal{B}1}\beta_{\mathcal{AB}}}{J_{10}}\lvert^{3}\mathrm{CT}^{10,-}_{\mathtt{B}};M_S\rangle\}$ | $-\frac{(c_{\mathcal{A}1}c_{\mathcal{B}1}\beta_{\mathcal{AB}})^2}{J_{10}}$ | |
| | | $\lvert^{1}\mathrm{LE}^{10,-}_{\mathtt{A}};0\rangle-\frac{c_{\mathcal{A}1}c_{\mathcal{B}1}\beta_{\mathcal{AB}}}{J_{10}+2K_{10}}\lvert^{1}\mathrm{CT}^{10,-}_{\mathtt{A}};0\rangle$ | $(1+c_{\mathcal{A}1}c_{\mathcal{A}1})\gamma_{\mathcal{AB}}$ | |
| | | $\lvert^{1}\mathrm{LE}^{10,-}_{\mathtt{B}};0\rangle+\frac{c_{\mathcal{A}1}c_{\mathcal{B}1}\beta_{\mathcal{AB}}}{J_{10}+2K_{10}}\lvert^{1}\mathrm{CT}^{-}_{\mathtt{B}};0\rangle$ | $-\frac{(c_{\mathcal{A}1}c_{\mathcal{B}1}\beta_{\mathcal{AB}})^2}{J_{10}+2K_{10}}$ | |
| $\{\lvert^{3}\mathrm{CT}^{10,P}_{\Gamma};M_S\rangle\,\lvert M_S,P,\Gamma\}$ | $E(\mathrm{LE}^-)+J_{10}$ | $\{\lvert^{3}\mathrm{CT}^{10,+}_{\mathtt{A}};M_S\rangle-\frac{c_{\mathcal{A}1}c_{\mathcal{B}1}\beta_{\mathcal{AB}}}{J_{10}-2K_{10}}\lvert^{3}\mathrm{LE}^{10,+}_{\mathtt{A}};M_S\rangle\,\lvert M_S\}$ | $E(\mathrm{LE}^-)+J_{10}$ | $\{\langle^{3}\mathrm{GS};M_S\rvert\,\boldsymbol{\mu}\,\lvert^{3}\mathrm{LE}^{10,+}_{\mathtt{A}};M_S\rangle\times\left(-\frac{c_{\mathcal{A}1}c_{\mathcal{B}1}\beta_{\mathcal{AB}}}{J_{10}-2K_{10}}\right)\lvert M_S\}$ |
| | | $\{\lvert^{3}\mathrm{CT}^{10,+}_{\mathtt{B}};M_S\rangle+\frac{c_{\mathcal{A}1}c_{\mathcal{B}1}\beta_{\mathcal{AB}}}{J_{10}-2K_{10}}\lvert^{3}\mathrm{LE}^{10,+}_{\mathtt{B}};M_S\rangle\,\lvert M_S\}$ | $+(1+c_{\mathcal{A}1}c_{\mathcal{A}1})\gamma_{\mathcal{AB}}+\frac{(c_{\mathcal{A}1}c_{\mathcal{B}1}\beta_{\mathcal{AB}})^2}{J_{10}-2K_{10}}$ | $\{\langle^{3}\mathrm{GS};M_S\rvert\,\boldsymbol{\mu}\,\lvert^{3}\mathrm{LE}^{10,+}_{\mathtt{B}};M_S\rangle\times\left(\frac{c_{\mathcal{A}1}c_{\mathcal{B}1}\beta_{\mathcal{AB}}}{J_{10}-2K_{10}}\right)\lvert M_S\}$ |
| | | $\{\lvert^{3}\mathrm{CT}^{10,-}_{\mathtt{A}};M_S\rangle-\frac{c_{\mathcal{A}1}c_{\mathcal{B}1}\beta_{\mathcal{AB}}}{J_{10}}\lvert^{3}\mathrm{LE}^{10,-}_{\mathtt{A}};M_S\rangle\,\lvert M_S\}$ | $E(\mathrm{LE}^-)+J_{10}$ | 0 |
| | | $\{\lvert^{3}\mathrm{CT}^{10,-}_{\mathtt{B}};M_S\rangle+\frac{c_{\mathcal{A}1}c_{\mathcal{B}1}\beta_{\mathcal{AB}}}{J_{10}}\lvert^{3}\mathrm{LE}^{10,-}_{\mathtt{B}};M_S\rangle\,\lvert M_S\}$ | $+(1+c_{\mathcal{A}1}c_{\mathcal{A}1})\gamma_{\mathcal{AB}}+\frac{(c_{\mathcal{A}1}c_{\mathcal{B}1}\beta_{\mathcal{AB}})^2}{J_{10}}$ | |
| $\{\lvert^{2S+1}\mathrm{LE}^{10,+}_{\Gamma};M_S\rangle\,\lvert S,M_S,\Gamma\}$ | $E(\mathrm{LE}^-)+2K_{10}$ | $\{\lvert^{3}\mathrm{LE}^{10,+}_{\mathtt{A}};M_S\rangle+\frac{c_{\mathcal{A}1}c_{\mathcal{B}1}\beta_{\mathcal{AB}}}{J_{10}-2K_{10}}\lvert^{3}\mathrm{CT}^{10,+}_{\mathtt{A}};M_S\rangle\,\lvert M_S\}$ | $E(\mathrm{LE}^-)+2K_{10}$ | $\{\langle^{2S+1}\mathrm{GS};M_S\rvert\,\boldsymbol{\mu}\,\lvert^{2S+1}\mathrm{LE}^{10,+}_{\Gamma};M_S\rangle$ |
| | | $\{\lvert^{3}\mathrm{LE}^{10,+}_{\mathtt{B}};M_S\rangle-\frac{c_{\mathcal{A}1}c_{\mathcal{B}1}\beta_{\mathcal{AB}}}{J_{10}-2K_{10}}\lvert^{3}\mathrm{CT}^{10,+}_{\mathtt{B}};M_S\rangle\,\lvert M_S\}$ | $+(1+c_{\mathcal{A}1}c_{\mathcal{A}1})\gamma_{\mathcal{AB}}-\frac{(c_{\mathcal{A}1}c_{\mathcal{B}1}\beta_{\mathcal{AB}})^2}{J_{10}-2K_{10}}$ | $\lvert S,M_S,\Gamma\}$ |
| | | $\lvert^{1}\mathrm{LE}^{10,+}_{\mathtt{A}};0\rangle-\frac{c_{\mathcal{A}1}c_{\mathcal{B}1}\beta_{\mathcal{AB}}}{J_{10}}\lvert^{1}\mathrm{CT}^{10,+}_{\mathtt{A}};0\rangle$ | $E(\mathrm{LE}^-)+2K_{10}$ | |
| | | $\lvert^{1}\mathrm{LE}^{10,+}_{\mathtt{B}};0\rangle+\frac{c_{\mathcal{A}1}c_{\mathcal{B}1}\beta_{\mathcal{AB}}}{J_{10}}\lvert^{1}\mathrm{CT}^{10,+}_{\mathtt{B}};0\rangle$ | $+(1+c_{\mathcal{A}1}c_{\mathcal{A}1})\gamma_{\mathcal{AB}}-\frac{(c_{\mathcal{A}1}c_{\mathcal{B}1}\beta_{\mathcal{AB}})^2}{J_{10}}$ | |
| $\{\lvert^{1}\mathrm{CT}^{10,P}_{\Gamma};0\rangle\,\lvert P,\Gamma\}$ | $E(\mathrm{LE}^-)+J_{10}+2K_{10}$ | $\lvert^{1}\mathrm{CT}^{10,-}_{\mathtt{A}};0\rangle+\frac{c_{\mathcal{A}1}c_{\mathcal{B}1}\beta_{\mathcal{AB}}}{J_{10}+2K_{10}}\lvert^{1}\mathrm{LE}^{10,-}_{\mathtt{A}};0\rangle$ | $E(\mathrm{LE}^-)+J_{10}+2K_{10}$ | 0 |
| | | $\lvert^{1}\mathrm{CT}^{10,-}_{\mathtt{B}};0\rangle-\frac{c_{\mathcal{A}1}c_{\mathcal{B}1}\beta_{\mathcal{AB}}}{J_{10}+2K_{10}}\lvert^{1}\mathrm{LE}^{10,-}_{\mathtt{B}};0\rangle$ | $+(1+c_{\mathcal{A}1}c_{\mathcal{A}1})\gamma_{\mathcal{AB}}+\frac{(c_{\mathcal{A}1}c_{\mathcal{B}1}\beta_{\mathcal{AB}})^2}{J_{10}+2K_{10}}$ | |
| | | $\lvert^{1}\mathrm{CT}^{10,+}_{\mathtt{A}};0\rangle+\frac{c_{\mathcal{A}1}c_{\mathcal{B}1}\beta_{\mathcal{AB}}}{J_{10}}\lvert^{1}\mathrm{LE}^{10,+}_{\mathtt{A}};0\rangle$ | $E(\mathrm{LE}^-)+J_{10}+2K_{10}$ | $\frac{c_{\mathcal{A}1}c_{\mathcal{B}1}\beta_{\mathcal{AB}}}{J_{10}}\langle^{1}\mathrm{GS};0\rvert\,\boldsymbol{\mu}\,\lvert^{1}\mathrm{LE}^{10,+}_{\mathtt{A}};0\rangle$ |
| | | $\lvert^{1}\mathrm{CT}^{10,+}_{\mathtt{B}};0\rangle-\frac{c_{\mathcal{A}1}c_{\mathcal{B}1}\beta_{\mathcal{AB}}}{J_{10}}\lvert^{1}\mathrm{LE}^{10,+}_{\mathtt{B}};0\rangle$ | $+(1+c_{\mathcal{A}1}c_{\mathcal{A}1})\gamma_{\mathcal{AB}}+\frac{(c_{\mathcal{A}1}c_{\mathcal{B}1}\beta_{\mathcal{AB}})^2}{J_{10}}$ | $-\frac{c_{\mathcal{A}1}c_{\mathcal{B}1}\beta_{\mathcal{AB}}}{J_{10}}\langle^{1}\mathrm{GS};0\rvert\,\boldsymbol{\mu}\,\lvert^{1}\mathrm{LE}^{10,+}_{\mathtt{B}};0\rangle$ |

## S4 Deriving the SOC operator for AHR $m$-dimers

Our derivation of the SOC operator for the PPP model closely follows that of Barford et al. [4]. We begin with the following effective one-electron Breit-Pauli Hamiltonian (in atomic units):

$$\hat{V}_{\text{SOC}} = \frac{1}{2c^2} \sum_j \sum_\mu \frac{Z_\mu^{\text{eff}}}{\hat{r}_{j\mu}^3} \hat{\mathbf{l}}_j^{(\mu)} \cdot \hat{\mathbf{s}}_j, \tag{S41}$$

where the indices $j$ and $\mu$ are summed over all electrons and nuclei respectively. Here, $\hat{\mathbf{l}}_j^{(\mu)}$ is the orbital angular momentum of electron $j$ with respect to nucleus $\mu$, separated by a distance $\hat{r}_{j\mu}$, and $\hat{\mathbf{s}}_j$ is the corresponding spin angular momentum. Also, $Z_\mu^{\text{eff}}$ is the effective nuclear charge of atom $\mu$ including screening effects by the two-electron Breit-Pauli terms and $c$ is the speed of light in vacuum. Within the minimal basis of $2p$ AOs being considered by the PPP formalism, we may restrict ourselves to the computation of the following matrix elements:

$$\left\langle 2p_{z'}^{(\mu')}; \sigma' \right| \frac{1}{2c^2} \sum_{\mu''} \frac{Z_{\mu''}^{\text{eff}}}{\hat{r}_{\mu''}^3} \hat{\mathbf{l}}^{(\mu'')} \cdot \hat{\mathbf{s}} \left| 2p_z^{(\mu)}; \sigma \right\rangle, \tag{S42}$$

where, in considering a specific electron $j$, we have omitted the electron index. The state $\left| 2p_z^{(\mu)}; \sigma \right\rangle$ denotes a spin-$\sigma$ electron occupying the $2p_z$ AO of atom $\mu$, with $z$ representing the orbital quantisation axis local to atom $\mu$. Due to the $1/r^3$ scaling, we assume the above integral to be zero unless $\mu$ and $\mu'$ represent the same or nearest-neighbour atom(s) and also assume the sum over $\mu''$ to be dominated by terms of $\mu'' \in \{\mu, \mu'\}$. Thus, the above integral vanishes when $\mu = \mu'$ (by evaluating its value explicitly) and the only matrix element we require is

$$A_{\mu\mu'} \equiv \left\langle 2p_{z'}^{(\mu')}; \sigma' \right| \frac{1}{c^2} \frac{Z_\mu^{\text{eff}}}{\hat{r}_\mu^3} \hat{\mathbf{l}}^{(\mu)} \cdot \hat{\mathbf{s}} \left| 2p_z^{(\mu)}; \sigma \right\rangle, \tag{S43}$$

with atoms $\mu$ and $\mu'$ being nearest-neighbours, such that

$$\left\langle 2p_{z'}^{(\mu')}; \sigma' \right| \frac{1}{2c^2} \sum_{\mu''} \frac{Z_{\mu''}^{\text{eff}}}{\hat{r}_{\mu''}^3} \hat{\mathbf{l}}^{(\mu'')} \cdot \hat{\mathbf{s}} \left| 2p_z^{(\mu)}; \sigma \right\rangle \approx \frac{A_{\mu\mu'}}{2} + \frac{A_{\mu'\mu}^*}{2}, \tag{S44}$$

where we have noted that $\hat{\mathbf{l}}^{(\mu)} \cdot \hat{\mathbf{s}} / \hat{r}_\mu^3$ is Hermitian. In general, the $z$-axis of atom $\mu$ may not coincide with the $z'$-axis of atom $\mu'$, instead having a component parallel to the $y'$-axis of atom $\mu'$ (if we align both $x$- and $x'$-axes to the vector connecting atom $\mu$ to atom $\mu'$). Therefore, for convenience, we rotate the coordinate system of atom $\mu$ so that the two atoms have parallel Cartesian axes. This is done by observing elements of the 3D rotation matrix for the $x$-axis and substituting

$$\left| 2p_z^{(\mu)}; \sigma \right\rangle = -\sin\theta_{\mu\mu'} \left| 2p_{y'}^{(\mu)}; \sigma \right\rangle + \cos\theta_{\mu\mu'} \left| 2p_{z'}^{(\mu)}; \sigma \right\rangle, \tag{S45}$$

where $\theta_{\mu\mu'}$ is the clockwise angle that the $z'$-axis makes relative to the $z$-axis. We also align the $z'$-axis to the spin axis so that we may easily evaluate the action of the components of $\hat{\mathbf{s}}$ on the spin orbitals. Because we expect the spin quantisation axis to be perpendicular to the $x$-axis (parallel to the dimer $C_2$ axis), we again use elements of the 3D rotation matrix for the $x$-axis and make the following substitutions:

$$\left| 2p_{y'}^{(\mu)}; \sigma \right\rangle = \cos\varphi \left| 2p_{y''}^{(\mu)}; \sigma \right\rangle + \sin\varphi \left| 2p_{z''}^{(\mu)}; \sigma \right\rangle, \tag{S46}$$

$$\left| 2p_{z'}^{(\mu)}; \sigma \right\rangle = -\sin\varphi \left| 2p_{y''}^{(\mu)}; \sigma \right\rangle + \cos\varphi \left| 2p_{z''}^{(\mu)}; \sigma \right\rangle, \tag{S47}$$

$$\left| 2p_{z'}^{(\mu')}; \sigma' \right\rangle = -\sin\varphi \left| 2p_{y''}^{(\mu')}; \sigma' \right\rangle + \cos\varphi \left| 2p_{z''}^{(\mu')}; \sigma' \right\rangle, \tag{S48}$$

with $z''$ representing the spin quantisation axis and $\varphi$ being the clockwise angle that the $z''$-axis makes relative to the $z'$-axis. From here, Eq. (S43) is easily evaluated by observing the matrix elements of $\hat{\mathbf{l}} \cdot \hat{\mathbf{s}}$ in the $2p$ AO basis (see, for instance, Ref. [4]). Because the following spatial integrals are equal:

$$\left(2p_{y''}^{(\mu')}\middle|\, \frac{Z_\mu^{\text{eff}}}{\hat{r}_\mu^3} \,\middle|2p_{y''}^{(\mu)}\right) = \left(2p_{z''}^{(\mu')}\middle|\, \frac{Z_\mu^{\text{eff}}}{\hat{r}_\mu^3} \,\middle|2p_{z''}^{(\mu)}\right) = \left(2p_{z}^{(\mu')}\middle|\, \frac{Z_\mu^{\text{eff}}}{\hat{r}_\mu^3} \,\middle|2p_{z}^{(\mu)}\right) \tag{S49}$$

due to invariance of $1/\hat{r}_\mu^3$ under rotation about the $x$-axis, we find $A_{\mu\mu'}$ to have the following result:

$$A_{\mu\mu'} = B_{\mu\mu'} \sin\left(\theta_{\mu\mu'}\right) \delta_{\sigma'\overline{\sigma}}, \tag{S50}$$

$$B_{\mu\mu'} \equiv -\frac{i}{2c^2} \left(2p_{z}^{(\mu')}\middle|\, \frac{Z_\mu^{\text{eff}}}{\hat{r}_\mu^3} \,\middle|2p_{z}^{(\mu)}\right), \tag{S51}$$

with no dependence on $\varphi$ ($\overline{\sigma}$ is the spin complementary to $\sigma$). Also, $A^*_{\mu'\mu} = A_{\mu\mu'}$ because (1) $\theta_{\mu\mu'} = -\theta_{\mu'\mu}$ and (2) $B_{\mu\mu'}$, being a purely imaginary number, equals $-B^*_{\mu'\mu}$. Therefore, overall, we find the SOC operator for the PPP model to be

$$\hat{V}_{\text{SOC}} = \sum_{\langle \mu,\mu' \rangle} B_{\mu\mu'} \sin\left(\theta_{\mu\mu'}\right) \left(\hat{a}^\dagger_{\mu\alpha}\hat{a}_{\mu'\beta} - \hat{a}^\dagger_{\mu'\beta}\hat{a}_{\mu\alpha}\right). \tag{S52}$$

Assuming AHRs to be planar, the only surviving terms in $\hat{V}_{\text{SOC}}$ for AHR $m$-dimer systems will be for $\mu, \mu' \in \{\mathcal{A}, \mathcal{B}\}$. This yields the following expression from the main text:

$$\hat{V}_{\text{SOC}} = \sum_{\sigma} B \sin\left(\theta\right) \left(\hat{a}^\dagger_{\mathcal{A}\sigma}\hat{a}_{\mathcal{B}\overline{\sigma}} - \hat{a}^\dagger_{\mathcal{B}\overline{\sigma}}\hat{a}_{\mathcal{A}\sigma}\right), \tag{S53}$$

where $\theta \equiv \theta_{\mathcal{AB}}$ is the torsional angle between the two AHRs and $B \equiv B_{\mathcal{AB}}$.

## S5 Results from configuration interaction between $\left|{}^3\mathbf{LE}_\Gamma^{10,+}; M_S\right\rangle$ and $\left|{}^3\mathbf{CT}_\Gamma^{10,+}; M_S\right\rangle$ states

When the $\left|{}^3\text{LE}_\Gamma^{10,+}; M_S\right\rangle$ and $\left|{}^3\text{CT}_\Gamma^{10,+}; M_S\right\rangle$ excitations are near-degenerate, off-diagonal matrix elements of the Hamiltonian $\hat{H} = \hat{H}_A + \hat{H}_B + \hat{V}_{AB}$ between these states cannot be ignored. Instead, we diagonalise the following configuration interaction matrix:

$$\mathbf{H}_{M_S,\Gamma} = \begin{pmatrix} \left\langle {}^3\text{LE}_\Gamma^{10,+}; M_S\middle|\, \hat{H} \,\middle|{}^3\text{LE}_\Gamma^{10,+}; M_S\right\rangle & \left\langle {}^3\text{LE}_\Gamma^{10,+}; M_S\middle|\, \hat{H} \,\middle|{}^3\text{CT}_\Gamma^{10,+}; M_S\right\rangle \\ \left\langle {}^3\text{CT}_\Gamma^{10,+}; M_S\middle|\, \hat{H} \,\middle|{}^3\text{LE}_\Gamma^{10,+}; M_S\right\rangle & \left\langle {}^3\text{CT}_\Gamma^{10,+}; M_S\middle|\, \hat{H} \,\middle|{}^3\text{CT}_\Gamma^{10,+}; M_S\right\rangle \end{pmatrix}, \tag{S54}$$

where we have noted that the full Hamiltonian matrix is block-diagonal in $M_S$ and $\Gamma$. Approximating $\hat{V}_{AB} \approx \hat{V}_{\text{NN}}$ and using values from Table S1, we obtain the following eigenfunctions:

$$\left|{}^3\left[\text{CT}+\text{LE}\right]_\Gamma^{10,+}; M_S\right\rangle = \cos\left(\frac{\phi}{2}\right)\left|{}^3\text{LE}_\Gamma^{10,+}; M_S\right\rangle + \sin\left(\frac{\phi}{2}\right)\left|{}^3\text{CT}_\Gamma^{10,+}; M_S\right\rangle, \tag{S55}$$

$$\left|{}^3\left[\text{CT}-\text{LE}\right]_\Gamma^{10,+}; M_S\right\rangle = -\sin\left(\frac{\phi}{2}\right)\left|{}^3\text{LE}_\Gamma^{10,+}; M_S\right\rangle + \cos\left(\frac{\phi}{2}\right)\left|{}^3\text{CT}_\Gamma^{10,+}; M_S\right\rangle, \tag{S56}$$

and energies

$$E\left({}^3\left[\text{CT}+\text{LE}\right]_\Gamma^{10,+}\right) = E\left(\text{LE}^-\right) + \left(1 + c^*_{\mathcal{A}1}c_{\mathcal{A}1}\right)\gamma_{\mathcal{AB}} + J_{10} + \frac{\Delta}{2} + \sqrt{\frac{\Delta^2}{4} + \left(c_{\mathcal{A}1}c_{\mathcal{B}1}\beta_{\mathcal{AB}}\right)^2}, \tag{S57}$$

$$E\left({}^3\left[\text{CT}-\text{LE}\right]_\Gamma^{10,+}\right) = E\left(\text{LE}^-\right) + \left(1 + c^*_{\mathcal{A}1}c_{\mathcal{A}1}\right)\gamma_{\mathcal{AB}} + J_{10} + \frac{\Delta}{2} - \sqrt{\frac{\Delta^2}{4} + \left(c_{\mathcal{A}1}c_{\mathcal{B}1}\beta_{\mathcal{AB}}\right)^2}, \tag{S58}$$

with detuning $\Delta$ and mixing angle $\phi$ defined as

$$\Delta \equiv 2K_{10} - J_{10}, \qquad \phi \equiv \tan^{-1}\left[\frac{-\chi_\Gamma\left(C_2\right) c_{\mathcal{A}1} c_{\mathcal{B}1} \beta_{\mathcal{AB}}}{\Delta/2}\right] \in (-\pi, \pi]. \tag{S59}$$

Here, $\chi_\Gamma\left(C_2\right)$ is the character of irrep $\Gamma$ for the $C_2$ operator, with

$$\chi_\Gamma\left(C_2\right) = \begin{cases} +1 & \Gamma = \mathtt{A}, \\ -1 & \Gamma = \mathtt{B}. \end{cases}$$

## S6 Deriving the energy expression for CS states

We find the energy expression for a CS state by expanding its determinant using $j_\pm \approx 2^{-1/2}\left(j_A \pm j_B\right)$:

$$|\mathrm{CS}\rangle \equiv \left|\cdots 1_+ \overline{1_+} 1_- \overline{1_-} 0_+ \overline{0_+}\right\rangle = \frac{1}{2} \sum_{r,r'=A,B} \left|\cdots 1_A \overline{1_A} \cdots 1_B \overline{1_B} 0_r \overline{0_{r'}}\right\rangle. \tag{S60}$$

For AHR $m$-dimers, the approximate Hamiltonian $\hat{H} \approx \hat{H}_A + \hat{H}_B + \hat{V}_{\mathrm{NN}}$ does not faciliate intermonomer excitations involving the SOMOs due to their nodal structures. Hence, when evaluating the energy expectation of $|\mathrm{CS}\rangle$, the cross terms vanish and we obtain

$$\langle \mathrm{CS}| \hat{H} |\mathrm{CS}\rangle \approx \frac{1}{2}\left(\left\langle\cdots 0_A \overline{0_A}\right| \hat{H} \left|\cdots 0_A \overline{0_A}\right\rangle + \left\langle\cdots 0_A \overline{0_B}\right| \hat{H} \left|\cdots 0_A \overline{0_B}\right\rangle\right), \tag{S61}$$

where we have noted that $\hat{H}$ is invariant under the $C_2$ unitary operation. Using standard electronic structure theory algebra [3], we find that

$$\left\langle\cdots 0_A \overline{0_A}\right| \hat{H} \left|\cdots 0_A \overline{0_A}\right\rangle - \left\langle\cdots 0_A \overline{0_B}\right| \hat{H} \left|\cdots 0_A \overline{0_B}\right\rangle = J_{00}, \tag{S62}$$

$$\left\langle {}^1\mathrm{GS}; 0\right| \hat{H} \left|{}^1\mathrm{GS}; 0\right\rangle \approx \left\langle\cdots 0_A \overline{0_B}\right| \hat{H} \left|\cdots 0_A \overline{0_B}\right\rangle, \tag{S63}$$

and noting $\left\langle {}^3\mathrm{GS}; 0\right| \hat{H} \left|{}^3\mathrm{GS}; 0\right\rangle \approx \left\langle {}^1\mathrm{GS}; 0\right| \hat{H} \left|{}^1\mathrm{GS}; 0\right\rangle$ from Table S1 yields

$$\langle \mathrm{CS}| \hat{H} |\mathrm{CS}\rangle \approx \left\langle {}^3\mathrm{GS}; 0\right| \hat{H} \left|{}^3\mathrm{GS}; 0\right\rangle + \frac{J_{00}}{2}, \tag{S64}$$

which is the expression in the main text.

# S7 Results from ab initio calculations of AHR $m$-dimers

## S7.1 Methylated benzylic radical $m$-dimer

### S7.1.1 DFT results

**Table S2**: Ground-state properties of the methylated benzylic radical $m$-dimer, calculated using DFT at the UB3LYP/6–31G(d,p) level.

| **Geometry** | **Optimised** ($\theta = 92.347^{\circ}$) | $\theta = 90.000^{\circ}$ | $\theta = 110.000^{\circ}$ |
|---|---|---|---|
| **Triplet** | | | |
| Energy / Hartree | –776.5671116713 | –776.5670703756 | –776.5651492072 |
| $\langle \mathbf{S}^2 \rangle$ | 2.069167388 | 2.069193399 | 2.068885009 |
| **BS** | | | |
| Energy / Hartree | | –776.5671567701 | –776.5653156632 |
| $\langle \mathbf{S}^2 \rangle$ | | 1.071306721 | 1.071552230 |
| **CS** | | | |
| Energy / Hartree | | –776.5295652419 | –776.5293547360 |
| $\langle \mathbf{S}^2 \rangle$ | | 0.000000000 | 0.000000000 |

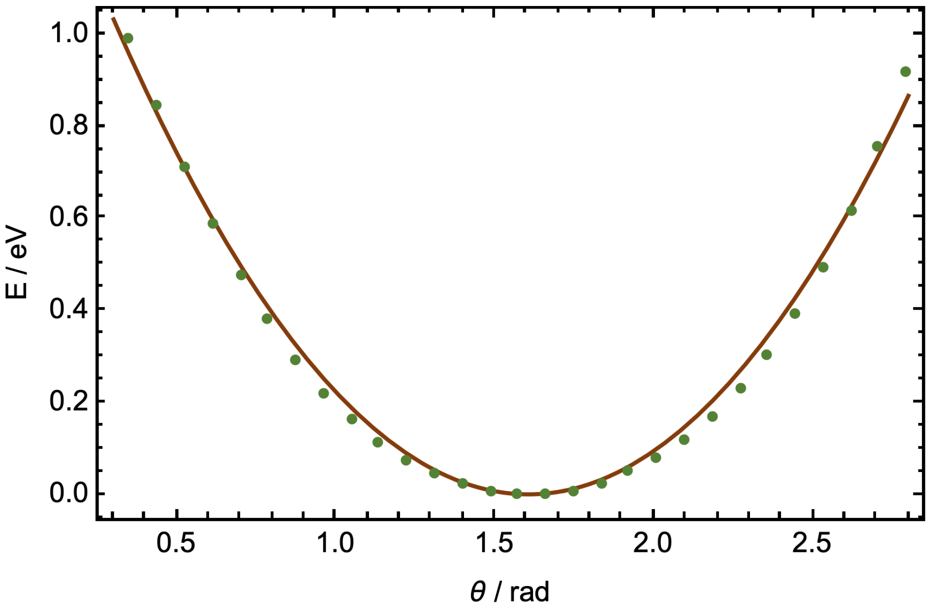


**FIG. S1**: Ground-state PES of the methylated benzylic radical $m$-dimer over different torsional angles $\theta$. (Green) Relative energies from a PES scan of the triplet configuration using DFT at the UB3LYP/6–31G(d,p) level. (Brown) Plot of $V_{\text{steric}}(\theta) = E_{\text{steric}}(\theta - \theta_{\text{eq}})^2$ using the fitted parameters of $E_{\text{steric}} = 0.606\,\text{eV}\,\text{rad}^{-1}$ and $\theta_{\text{eq}} = 1.605$ rad.

**Optimised geometry** ($\theta = 92.347^{\circ}$)

```
C
C 1 1.409368
```

```
C 1 1.441059 2 116.340956
C 3 1.401527 1 120.070634 2 15.202939 0
H 4 1.087988 3 118.341091 1 175.683527 0
C 4 1.382896 3 122.997361 1 -9.117845 0
C 6 1.433807 4 118.274331 3 -0.726817 0
C 7 1.401193 6 120.026492 4 -176.084995 0
H 8 1.080866 7 122.456139 6 178.933076 0
H 8 1.082035 7 121.072888 6 0.063847 0
C 6 1.506883 4 120.175026 3 -178.597849 0
H 11 1.092955 6 110.715186 4 -2.994127 0
H 11 1.096680 6 111.774410 4 -123.236227 0
H 11 1.096908 6 111.713183 4 117.134509 0
C 1 1.511803 2 124.774624 3 -153.713020 0
C 15 1.409346 1 124.777118 2 19.999997 0
C 15 1.441080 1 114.006582 2 -134.241430 0
C 17 1.401508 15 120.070820 1 171.734601 0
H 18 1.087986 17 118.342080 15 175.685206 0
C 18 1.382915 17 122.996491 15 -9.115603 0
C 20 1.433796 18 118.274351 17 -0.733019 0
C 21 1.401196 20 120.026201 18 -176.076942 0
H 22 1.080866 21 122.455975 20 178.929019 0
H 22 1.082035 21 121.072902 20 0.060727 0
C 20 1.506883 18 120.174930 17 -178.599386 0
H 25 1.092955 20 110.715266 18 -2.999552 0
H 25 1.096680 20 111.774380 18 -123.241474 0
H 25 1.096909 20 111.713426 18 117.129123 0
C 17 1.516466 15 123.125798 1 1.968581 0
H 29 1.089739 17 115.467470 15 -51.719423 0
H 29 1.093907 17 110.425507 15 -174.558522 0
H 29 1.097909 17 109.273136 15 67.763138 0
C 3 1.516474 1 123.135737 2 -154.546153 0
H 33 1.089702 3 115.472708 1 -51.480275 0
H 33 1.093917 3 110.430699 1 -174.337781 0
H 33 1.097933 3 109.262519 1 67.998117 0
C 16 1.517329 15 120.487495 1 29.233221 0
H 37 1.089055 16 111.663034 15 -2.551472 0
H 37 1.095417 16 112.722561 15 -124.139845 0
H 37 1.095950 16 109.749322 15 117.043730 0
C 2 1.517329 1 120.487316 3 -177.051349 0
H 41 1.089051 2 111.663928 1 -2.563660 0
H 41 1.095415 2 112.722805 1 -124.153865 0
H 41 1.095953 2 109.747978 1 117.030713 0
```

**Geometry at $\theta = 90.000^{\mathbf{o}}$**

```
C
C  1 1.399552
C  1 1.418419 2 120.253895
C  3 1.402188 1 118.900634 2 0.164518 0
H  4 1.088026 3 118.440872 1 -179.909128 0
C  4 1.385963 3 122.796421 1 -0.067502 0
C  6 1.437187 4 119.111578 3 0.032632 0
```

```
C  7 1.402242 6 120.476927 4 -180.000000 0
H  8 1.081467 7 121.983110 6 179.984734 0
H  8 1.082068 7 121.397085 6 0.060852 0
C  1 1.506072 2 121.038541 3 -179.857867 0
C  11 1.399553 1 121.038670 2 90.000001 0
C  11 1.418420 1 118.707332 2 -89.860545 0
C  13 1.402188 11 118.900646 1 -179.976053 0
H  14 1.088026 13 118.440862 11 -179.907273 0
C  14 1.385963 13 122.796447 11 -0.065992 0
C  16 1.437187 14 119.111573 13 0.032888 0
C  17 1.402242 16 120.476842 14 179.998723 0
H  18 1.081467 17 121.983225 16 179.984860 0
H  18 1.082068 17 121.397007 16 0.060756 0
C  6 1.508194 4 119.889099 3 -179.938509 0
H  21 1.092897 6 110.826282 4 0.009973 0
H  21 1.096838 6 111.741943 4 -120.150420 0
H  21 1.096885 6 111.801511 4 120.191184 0
C  16 1.508194 14 119.889099 13 -179.938123 0
H  25 1.092897 16 110.826298 14 0.013292 0
H  25 1.096838 16 111.741962 14 -120.147137 0
H  25 1.096884 16 111.801379 14 120.194496 0
C  3 1.509316 1 121.444807 2 -178.917156 0
H  29 1.093360 3 110.799597 1 -177.225860 0
H  29 1.095928 3 112.118801 1 -56.517698 0
H  29 1.096637 3 111.692286 1 62.544234 0
C  13 1.509317 11 121.444868 1 0.941061 0
H  33 1.093360 13 110.799465 11 -177.229045 0
H  33 1.095929 13 112.118187 11 -56.521644 0
H  33 1.096636 13 111.692779 11 62.540325 0
C  2 1.510815 1 120.956022 3 -179.978450 0
H  37 1.089506 2 111.588571 1 -0.997702 0
H  37 1.096564 2 111.284282 1 -121.544604 0
H  37 1.096873 2 111.215588 1 119.628989 0
C  12 1.510815 11 120.956186 1 0.164869 0
H  41 1.089507 12 111.588891 11 -1.000241 0
H  41 1.096563 12 111.284382 11 -121.547634 0
H  41 1.096873 12 111.215335 11 119.626152 0
```

**Geometry at** $\theta = 110.000^{\mathbf{o}}$

```
C
C  1 1.400611
C  1 1.420229 2 119.944080
C  3 1.403111 1 118.869523 2 -1.925929 0
H  4 1.087964 3 118.350547 1 -179.877467 0
C  4 1.385002 3 122.978926 1 0.857552 0
C  6 1.437137 4 119.018082 3 0.099275 0
C  7 1.402315 6 120.503771 4 -179.958207 0
H  8 1.081357 7 122.003550 6 -179.944770 0
H  8 1.082081 7 121.400903 6 0.010622 0
C  1 1.506656 2 121.061967 3 173.919544 0
C  11 1.400612 1 121.060588 2 110.000002 0
```

```
C  11 1.420228 1 118.721760 2 -76.009871 0
C  13 1.403112 11 118.869420 1 -175.984045 0
H  14 1.087964 13 118.350711 11 -179.878235 0
C  14 1.385002 13 122.978879 11 0.857583 0
C  16 1.437137 14 119.018232 13 0.098808 0
C  17 1.402315 16 120.503677 14 -179.959065 0
H  18 1.081356 17 122.003377 16 -179.943542 0
H  18 1.082081 17 121.400899 16 0.011457 0
C  6 1.508012 4 119.932375 3 179.800301 0
H  21 1.092994 6 110.794216 4 -0.356820 0
H  21 1.096629 6 111.747082 4 -120.535327 0
H  21 1.096974 6 111.788535 4 119.790702 0
C  16 1.508012 14 119.932439 13 179.799081 0
H  25 1.092993 16 110.794314 14 -0.359195 0
H  25 1.096629 16 111.746989 14 -120.537687 0
H  25 1.096974 16 111.788594 14 119.788492 0
C  3 1.509711 1 122.015181 2 177.751454 0
H  29 1.093649 3 110.637404 1 -164.724957 0
H  29 1.093873 3 111.954366 1 -43.794978 0
H  29 1.097182 3 111.764383 1 75.774881 0
C  13 1.509713 11 122.015499 1 3.692891 0
H  33 1.093648 13 110.637081 11 -164.723187 0
H  33 1.093872 13 111.954262 11 -43.793214 0
H  33 1.097181 13 111.764472 11 75.776579 0
C  12 1.511105 11 120.778261 1 -6.759416 0
H  37 1.089670 12 111.555612 11 1.313032 0
H  37 1.096699 12 111.618461 11 122.346732 0
H  37 1.096805 12 110.970783 11 -118.836401 0
C  2 1.511107 1 120.778625 3 179.322947 0
H  41 1.089670 2 111.556325 1 1.321094 0
H  41 1.096698 2 111.618416 1 122.355288 0
H  41 1.096806 2 110.970469 1 -118.828184 0
```

### S7.1.2 MCSCF/CI results

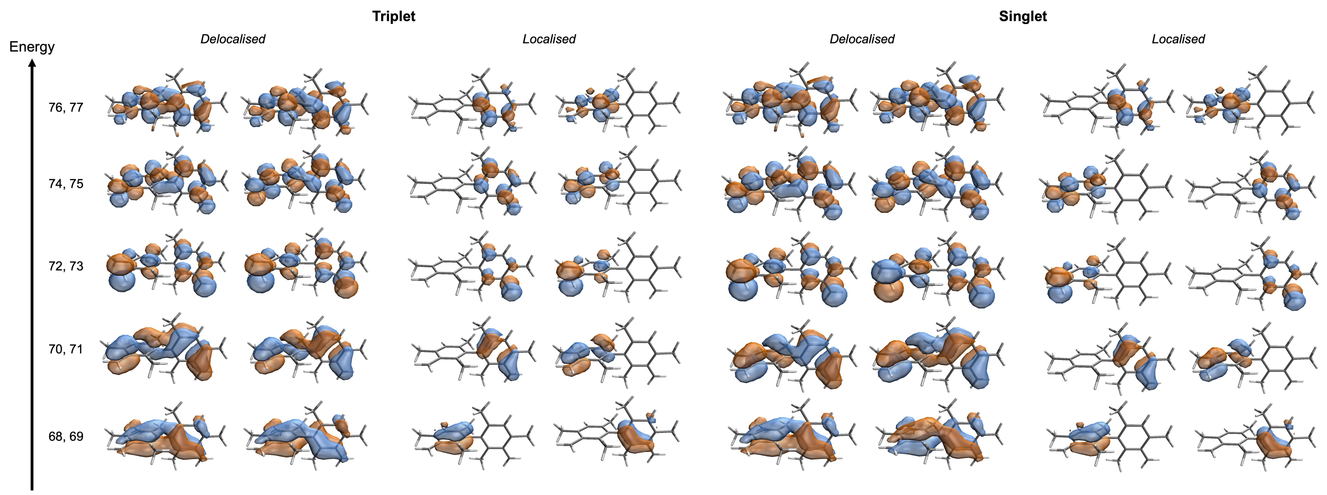


**FIG. S2**: Active space MOs of the methylated benzylic radical *m*-dimer from a state-specific CASSCF(10,10)/6–31G(d,p) calculation of the triplet and singlet ground states using the UB3LYP-optimised triplet ground-state geometry ($\theta = 92.347^{o}$). Delocalised MOs are MOs obtained directly from a CASSCF(10,10) calculation (isovalue = 0.030). Mixing each consecutive pair of MOs equally yields spatially localised MOs (isovalue = 0.060). MOs are arranged in increasing order of energy.

**Table S3**: Excited-state properties of the methylated benzylic radical *m*-dimer, calculated at the state-specific CASSCF(10,10)/CASCI/QD-SC-NEVPT2/6–31G(d,p) level using the UB3LYP-optimised triplet ground-state geometry ($\theta = 92.347^{o}$). Each excitation was assigned a state $\Phi_{\Gamma}^{j0,P}$. The class $\Phi \in \{\mathrm{GS}, \mathrm{LE}, \mathrm{CT}\}$ and orbital $j = 1, 2, \cdots$ were found by observing the dominant contributions to the CI vector in the spatially localised orbital basis [Fig. S2]. The particle-hole symmetry $P \in \{+, -\}$ was labelled based on the oscillator strengths, with $P = +$ states being significantly brighter than $P = -$ states; see Table S1. Because the triplet states at around 4.2 eV were dominated by both $1 \rightarrow 0$ and $2 \rightarrow 0$ CT transitions with little contributions from $0 \rightarrow 1'$ and $0 \rightarrow 2'$ CT transitions, no particle-hole symmetry was assigned. These results are not surprising since the $\mathrm{CT}^{j0,+}$ and $\mathrm{CT}^{j0,-}$ excitations are near-degenerate when $\theta \approx 90^{o}$ [Fig. 2c].

| Triplets | | | Singlets | | |
|---|---|---|---|---|---|
| **Energy / eV** | **Oscillator strength** | **Assignment** | **Energy / eV** | **Oscillator strength** | **Assignment** |
| 0 | – | GS | –0.005 | – | GS |
| 3.164 | 0.0153 | $\mathrm{LE}^{10,-}$ | 2.223 | 0.0000 | $\mathrm{CT}^{00}$ |
| 3.168 | 0.0097 | $\mathrm{LE}^{10,-}$ | 2.226 | 0.0016 | $\mathrm{CT}^{00}$ |
| 3.779 | 0.0185 | $\mathrm{LE}^{20,-}$ | 3.164 | 0.0096 | $\mathrm{LE}^{10,-}$ |
| 3.789 | 0.0039 | $\mathrm{LE}^{20,-}$ | 3.167 | 0.0170 | $\mathrm{LE}^{10,-}$ |
| 4.180 | 0.0058 | $\mathrm{CT}^{1\rightarrow 0}$ & $\mathrm{CT}^{2\rightarrow 0}$ | 3.788 | 0.0048 | $\mathrm{LE}^{20,-}$ |
| 4.191 | 0.0007 | $\mathrm{CT}^{1\rightarrow 0}$ & $\mathrm{CT}^{2\rightarrow 0}$ | 3.793 | 0.0185 | $\mathrm{LE}^{20,-}$ |
| 4.317 | 0.1369 | $\mathrm{LE}^{10,+}$ & $\mathrm{LE}^{20,+}$ | 4.326 | 0.1404 | $\mathrm{LE}^{10,+}$ & $\mathrm{LE}^{20,+}$ |
| 4.347 | 0.1413 | $\mathrm{LE}^{10,+}$ & $\mathrm{LE}^{20,+}$ | 4.343 | 0.1486 | $\mathrm{LE}^{10,+}$ & $\mathrm{LE}^{20,+}$ |

### S7.1.3 SOC matrix elements

**Table S4**: SOC matrix elements between close-lying (within 0.4 eV) electronic states of the methylated benzylic radical *m*-dimer. These calculations were performed at the CASCI/QD-SC-NEVPT2/6–31G(d,p) level using the UB3LYP-optimised triplet ground-state geometry ($\theta = 92.347^{\circ}$) and orbitals from CASSCF(10,10) state-specific to the triplet ground state. Excitations were assigned in the same way as Table S3 and the labels "(1)" and "(2)" indicate the lower and higher energy state of a particular excitation type. Note that the triplet magnetic sublevels are presented in the eigenbasis of $\hat{S}_z$, with the $z$-axis coinciding with the molecular $C_2$ axis. Matrix elements larger than $0.1\,\mathrm{cm}^{-1}$ in magnitude are presented in bold.

| **Triplet** | **Singlet** | **SOC magnitude / cm$^{-1}$** | | **Triplet** | **Singlet** | **SOC magnitude / cm$^{-1}$** | |
|---|---|---|---|---|---|---|---|
| | | $M_S = \pm1$ | $M_S = 0$ | | | $M_S = \pm1$ | $M_S = 0$ |
| GS | GS | 0.001 | 0.000 | | | | |
| LE$^{10,-}$ (1) | LE$^{10,-}$ (1) | 0.001 | 0.001 | LE$^{10,-}$ (2) | LE$^{10,-}$ (1) | 0.004 | 0.000 |
| LE$^{10,-}$ (1) | LE$^{10,-}$ (2) | 0.011 | 0.000 | LE$^{10,-}$ (2) | LE$^{10,-}$ (2) | 0.000 | 0.014 |
| LE$^{20,-}$ (1) | LE$^{20,-}$ (1) | 0.001 | 0.005 | LE$^{20,-}$ (2) | LE$^{20,-}$ (1) | 0.016 | 0.000 |
| LE$^{20,-}$ (1) | LE$^{20,-}$ (2) | 0.043 | 0.000 | LE$^{20,-}$ (2) | LE$^{20,-}$ (2) | 0.000 | 0.002 |
| CT$^{1\to0}$ & CT$^{2\to0}$ (1) | LE$^{20,-}$ (1) | 0.005 | 0.099 | CT$^{1\to0}$ & CT$^{2\to0}$ (2) | LE$^{20,-}$ (1) | **0.234** | 0.004 |
| CT$^{1\to0}$ & CT$^{2\to0}$ (1) | LE$^{20,-}$ (2) | **0.236** | 0.002 | CT$^{1\to0}$ & CT$^{2\to0}$ (2) | LE$^{20,-}$ (2) | 0.007 | 0.059 |
| CT$^{1\to0}$ & CT$^{2\to0}$ (1) | LE$^{10,+}$ & LE$^{20,+}$ (1) | 0.001 | 0.007 | CT$^{1\to0}$ & CT$^{2\to0}$ (2) | LE$^{10,+}$ & LE$^{20,+}$ (1) | **0.159** | 0.001 |
| CT$^{1\to0}$ & CT$^{2\to0}$ (1) | LE$^{10,+}$ & LE$^{20,+}$ (2) | **0.126** | 0.000 | CT$^{1\to0}$ & CT$^{2\to0}$ (2) | LE$^{10,+}$ & LE$^{20,+}$ (2) | 0.010 | 0.009 |
| LE$^{10,+}$ & LE$^{20,+}$ (1) | LE$^{10,+}$ & LE$^{20,+}$ (1) | 0.062 | 0.003 | LE$^{10,+}$ & LE$^{20,+}$ (2) | LE$^{10,+}$ & LE$^{20,+}$ (1) | 0.032 | 0.014 |
| LE$^{10,+}$ & LE$^{20,+}$ (1) | LE$^{10,+}$ & LE$^{20,+}$ (2) | 0.021 | 0.015 | LE$^{10,+}$ & LE$^{20,+}$ (2) | LE$^{10,+}$ & LE$^{20,+}$ (2) | 0.007 | 0.006 |

**Table S5**: Selected SOC matrix elements involving the GSs and $^1$CT$^{00}$ states of the methylated benzylic radical *m*-dimer. See Table S4 for computational details.

| **Triplet** | **Singlet** | **SOC magnitude / cm$^{-1}$** $M_S = \pm1$ | $M_S = 0$ | **Triplet** | **Singlet** | **SOC magnitude / cm$^{-1}$** $M_S = \pm1$ | $M_S = 0$ |
|---|---|---|---|---|---|---|---|
| GS | CT$^{00}$ (1) | 0.016 | 0.002 | GS | CT$^{00}$ (2) | 0.001 | 0.061 |
| CT$^{1\to0}$ & CT$^{2\to0}$ (1) | GS | 0.008 | **0.409** | CT$^{1\to0}$ & CT$^{2\to0}$ (2) | GS | **0.297** | 0.013 |
| LE$^{10,-}$ (1) | CT$^{00}$ (1) | 0.012 | 0.018 | LE$^{10,-}$ (2) | CT$^{00}$ (1) | 0.025 | 0.016 |
| LE$^{10,-}$ (1) | CT$^{00}$ (2) | **0.339** | 0.001 | LE$^{10,-}$ (2) | CT$^{00}$ (2) | 0.001 | **0.437** |

**Table S6**: SOC matrix elements between the $^1$LE$^{10,-}$ states and CT$^{1\to0}$ & CT$^{2\to0}$ states of the methylated benzylic radical *m*-dimer. See Table S4 for computational details.

| **Triplet** | **Singlet** | **SOC magnitude / cm$^{-1}$** $M_S = \pm1$ | $M_S = 0$ | **Triplet** | **Singlet** | **SOC magnitude / cm$^{-1}$** $M_S = \pm1$ | $M_S = 0$ |
|---|---|---|---|---|---|---|---|
| CT$^{1\to0}$ & CT$^{2\to0}$ (1) | LE$^{10,-}$ (1) | 0.005 | 0.071 | CT$^{1\to0}$ & CT$^{2\to0}$ (2) | LE$^{10,-}$ (1) | **0.165** | 0.003 |
| CT$^{1\to0}$ & CT$^{2\to0}$ (1) | LE$^{10,-}$ (2) | **0.163** | 0.001 | CT$^{1\to0}$ & CT$^{2\to0}$ (2) | LE$^{10,-}$ (2) | 0.008 | 0.064 |

We first analysed the SOC matrix elements between states separated in energy by $< 0.4$ eV (approximately one vibrational quantum) [Table S4]. These are also states among which ISC processes are most probable [5]. Indeed, CT-type transitions involving the triplet $M_S = \pm 1$ sublevels experienced the largest SOC matrix elements, dominating others by at least an order of magnitude. Furthermore, for each excitation containing two near-degenerate states of opposite irreps (labelled "(1)" and "(2)"), SOC matrix elements were selective for one of the two irreps. All these observations are consistent with the predictions made by the PPP model. Unfortunately, because the $\mathrm{CT}^{10}$ and $\mathrm{CT}^{20}$ excitations were not computed with definite particle-hole symmetry, selection rules for this property could not be verified.

Next, we tabulated the SOC matrix elements for CT-type transitions of the GSs and ${}^1\mathrm{CT}^{00}$ states [Table S5]. Interestingly, significant couplings were observed to some higher-lying states despite the SOMO having a node at the dimer linkage. In two cases, spin selectivity was even reversed to become $\Delta M_S = 0$. One explanation could be the presence of through-space spin-orbit interactions between electrons in $2p$ AOs that are spatially close but not adjacent to each other on the nuclear framework. Such effects can mix triplet $M_S = 0$ sublevels [6] and are not captured by the PPP model, which assumes nearest-neighbour coupling (i.e. only through-bond effects). Fortunately for us, the GSs and ${}^1\mathrm{CT}^{00}$ states are energetically separated from other excitations by at least 0.8 eV (around two vibrational quanta), so ISC processes of these states are likely to be slow [5]. As such, their impact on the accumulation of ground-state spin polarisation is likely to be small.

Pertaining to the spin polarisation mechanisms described in the main text, three sets of SOC matrix elements are particularly relevant:

a. For case 1 of ODMR in AHR $m$-dimers [Fig. 2d], the $\left|{}^3\mathrm{CT}^{10,+}\right\rangle \to \left|{}^1\mathrm{LE}^{10,+}\right\rangle$ ISC causes accumulation of spin polarisation. Their SOC matrix elements are presented in green in Table S4 and indeed, we find nearly 100% selectivity for the $M_S = \pm 1$ components of the ${}^3\mathrm{CT}^{10}$ excited states, in agreement with the PPP model.

b. As for case 2 of ODMR in AHR $m$-dimers [Fig. 2e], the $\left|{}^3\mathrm{CT}^{10,-}\right\rangle \to \left|{}^1\mathrm{LE}^{10,-}\right\rangle$ ISC causes accumulation of spin polarisation. These matrix elements are presented in Table S6 and also display close to 100% spin selectivity for the $M_S = \pm 1$ components of the ${}^3\mathrm{CT}^{10}$ excited state, in line with the PPP model.

c. Specific to the methylated benzylic radical $m$-dimer [Fig. 5b], MCSCF/CI calculations place this system in case 2. However, the ${}^1\mathrm{LE}^{10,-}$ states are $> 1$ eV lower in energy than the ${}^3\mathrm{CT}^{10}$ states, suggesting that ISC through this pathway is energetically disfavoured [5]. Instead, ISC is likely to occur to the closer-lying (0.39 eV) ${}^1\mathrm{LE}^{20,-}$ state, which is not an issue because the selection rules derived from the PPP model are generalisable to higher-lying LE and CT excitations. The $\left|{}^3\mathrm{CT}^{10,-}\right\rangle \to \left|{}^1\mathrm{LE}^{20,-}\right\rangle$ matrix elements are tabulated in red in Table S4. Again, we find these ISC processes to also be almost 100% selective for the $M_S = \pm 1$ components of the ${}^3\mathrm{CT}^{10}$ excited state, as predicted by the PPP framework.

### S7.2 TTM $m$-dimer

**Table S7**: Ground-state properties of the TTM $m$-dimer, calculated using DFT at the UB3LYP/6–31G(d,p) level.

| **Geometry** | **Optimised** ($\theta = 94.022^{o}$) | $\theta = 90.000^{o}$ | $\theta = 110.000^{o}$ |
|---|---|---|---|
| **Triplet** | | | |
| Energy / Hartree | –9737.4945065361 | –9737.4945443297 | –9737.4932288687 |
| $\langle \mathbf{S}^2 \rangle$ | 2.040030882 | 2.039735356 | 2.039988794 |
| **BS** | | | |
| Energy / Hartree | | –9737.4960015921 | –9737.49408829 |
| $\langle \mathbf{S}^2 \rangle$ | | 1.034521264 | 1.0312 |
| **CS** | | | |
| Energy / Hartree | | –9737.4566476404 | –9737.4557726141 |
| $\langle \mathbf{S}^2 \rangle$ | | –0.000000000 | –0.000000000 |

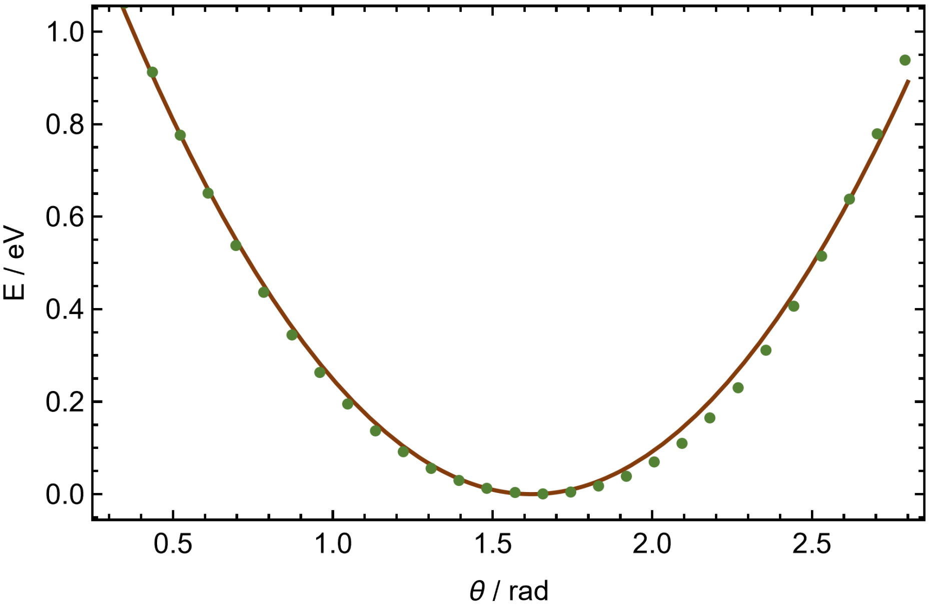


**FIG. S3**: Ground-state PES of the TTM $m$-dimer over different torsional angles $\theta$. (Green) Relative energies from a PES scan of the triplet configuration using DFT at the UB3LYP/6–31G(d,p) level. (Brown) Plot of $V_{\text{steric}}(\theta) = E_{\text{steric}}(\theta - \theta_{\text{eq}})^2$ using the fitted parameters of $E_{\text{steric}} = 0.643\,\text{eV}\,\text{rad}^{-1}$ and $\theta_{\text{eq}} = 1.622$ rad.

**Optimised geometry** ($\theta = 94.022^{o}$)

```
Cl
C  1 1.751799
C  2 1.402938 1 116.601767
C  3 1.401602 2 117.373233 1 -175.977144 0
C  4 1.389046 3 121.497716 2 0.146928 0
H  5 1.082109 4 120.359912 3 -179.125979 0
C  5 1.388134 4 119.435924 3 -0.487427 0
```

```
C  7 1.416077 5 122.756338 4 0.196756 0
C  8 1.476804 7 122.254762 5 -179.575975 0
C  9 1.473664 8 119.954750 7 -49.701863 0
C  10 1.419428 9 122.587078 8 131.180403 0
C  11 1.390522 10 123.263292 9 179.713317 0
H  12 1.082217 11 120.139706 10 178.956896 0
C  12 1.390762 11 118.962200 10 0.306325 0
C  14 1.390683 12 120.866310 11 -0.077919 0
H  15 1.082316 14 120.924838 12 -178.931241 0
C  15 1.390861 14 118.979806 12 -0.206287 0
C  9 1.474298 8 119.952018 7 129.893971 0
C  18 1.419160 9 122.633366 8 131.368734 0
C  19 1.390816 18 123.269670 9 -179.332712 0
H  20 1.082238 19 120.115031 18 178.756533 0
C  20 1.390556 19 118.977700 18 0.197707 0
C  22 1.390489 20 120.838307 19 -0.426246 0
H  23 1.082238 22 120.887786 20 -178.753937 0
C  23 1.390874 22 118.978963 20 0.052299 0
C  3 1.493059 2 121.712421 1 3.709171 0
C  26 1.401602 3 120.913591 2 85.653680 0
C  27 1.389046 26 121.497716 3 -179.542036 0
H  28 1.082109 27 120.359912 26 -179.125979 0
C  28 1.388134 27 119.435924 26 -0.487427 0
C  26 1.402938 3 121.712421 2 -94.021634 0
C  30 1.416077 28 122.756338 27 0.196756 0
C  32 1.476804 30 122.254762 28 -179.575975 0
C  33 1.473664 32 119.954750 30 -49.701863 0
C  34 1.419428 33 122.587078 32 131.180403 0
C  35 1.390522 34 123.263292 33 179.713317 0
H  36 1.082217 35 120.139706 34 178.956896 0
C  36 1.390762 35 118.962200 34 0.306325 0
C  38 1.390683 36 120.866310 35 -0.077919 0
H  39 1.082316 38 120.924838 36 -178.931241 0
C  39 1.390861 38 118.979806 36 -0.206287 0
C  33 1.474298 32 119.952019 30 129.893971 0
C  42 1.419160 33 122.633366 32 131.368734 0
C  43 1.390816 42 123.269670 33 -179.332712 0
H  44 1.082238 43 120.115031 42 178.756533 0
C  44 1.390556 43 118.977700 42 0.197707 0
C  46 1.390489 44 120.838307 43 -0.426246 0
H  47 1.082238 46 120.887786 44 -178.753937 0
C  47 1.390874 46 118.978963 44 0.052299 0
Cl 27 1.748625 26 120.416165 3 0.504861 0
Cl 4 1.748625 3 120.416165 2 -179.806175 0
Cl 38 1.749533 36 119.527040 35 179.814910 0
Cl 14 1.749533 12 119.527040 11 179.814910 0
Cl 46 1.750108 44 119.579778 43 179.428546 0
Cl 22 1.750108 20 119.579778 19 179.428546 0
Cl 31 1.751799 26 116.601767 3 3.709171 0
Cl 30 1.752882 28 115.706988 27 -176.366242 0
Cl 7 1.752882 5 115.706988 4 -176.366242 0
Cl 41 1.753764 39 115.582866 38 -176.333728 0
Cl 17 1.753764 15 115.582866 14 -176.333728 0
```

```
Cl 49 1.754031 47 115.506561 46 -176.120010 0
Cl 25 1.754031 23 115.506561 22 -176.120010 0
Cl 43 1.754332 42 121.158698 33 -3.202799 0
Cl 19 1.754332 18 121.158698 9 -3.202799 0
Cl 35 1.754804 34 121.157263 33 -4.092130 0
Cl 11 1.754804 10 121.157263 9 -4.092130 0
```

**Geometry at** $\theta = 90.000^{\mathbf{o}}$

```
Cl
C  1 1.751771
C  2 1.403211 1 116.633814
C  3 1.401377 2 117.319593 1 -176.273522 0
C  4 1.388983 3 121.533456 2 0.007214 0
H  5 1.082160 4 120.346860 3 -179.164590 0
C  5 1.388212 4 119.436003 3 -0.324343 0
C  7 1.415901 5 122.728780 4 0.003478 0
C  8 1.477314 7 122.223695 5 -179.460654 0
C  9 1.474226 8 119.873546 7 -49.920770 0
C  10 1.419135 9 122.695318 8 -49.282987 0
C  11 1.390926 10 123.190200 9 -179.982110 0
H  12 1.082347 11 120.102480 10 178.962500 0
C  12 1.390647 11 118.987133 10 0.211249 0
C  14 1.390785 12 120.893495 11 -0.199114 0
H  15 1.082215 14 120.905253 12 -178.735772 0
C  15 1.390531 14 118.913074 12 -0.022696 0
C  9 1.474285 8 120.053381 7 129.678484 0
C  18 1.419140 9 122.712252 8 -48.137716 0
C  19 1.390823 18 123.292027 9 178.914751 0
H  20 1.082182 19 120.129393 18 179.342068 0
C  20 1.390386 19 118.958691 18 0.552351 0
C  22 1.390551 20 120.839712 19 0.063836 0
H  23 1.082241 22 120.856549 20 -179.102304 0
C  23 1.390794 22 118.999400 20 -0.418080 0
C  3 1.493689 2 121.712442 1 2.280919 0
C  26 1.401377 3 120.951894 2 88.502409 0
C  27 1.388983 26 121.533456 3 -178.558864 0
H  28 1.082160 27 120.346860 26 -179.164590 0
C  28 1.388212 27 119.436003 26 -0.324343 0
C  26 1.403211 3 121.712442 2 -90.000002 0
C  30 1.415901 28 122.728780 27 0.003478 0
C  32 1.477314 30 122.223695 28 -179.460654 0
C  33 1.474226 32 119.873546 30 -49.920770 0
C  34 1.419135 33 122.695318 32 -49.282987 0
C  35 1.390926 34 123.190200 33 -179.982110 0
H  36 1.082347 35 120.102480 34 178.962500 0
C  36 1.390647 35 118.987133 34 0.211249 0
C  38 1.390785 36 120.893495 35 -0.199114 0
H  39 1.082215 38 120.905253 36 -178.735772 0
C  39 1.390531 38 118.913074 36 -0.022696 0
C  33 1.474285 32 120.053381 30 129.678484 0
C  42 1.419140 33 122.712252 32 -48.137716 0
```

```
C  43 1.390823 42 123.292027 33 178.914751 0
H  44 1.082182 43 120.129393 42 179.342068 0
C  44 1.390386 43 118.958691 42 0.552351 0
C  46 1.390551 44 120.839712 43 0.063836 0
H  47 1.082241 46 120.856549 44 -179.102304 0
C  47 1.390794 46 118.999400 44 -0.418080 0
Cl 27 1.748894 26 120.377826 3 1.262758 0
Cl 4 1.748894 3 120.377826 2 179.828836 0
Cl 38 1.749671 36 119.580222 35 179.877116 0
Cl 14 1.749671 12 119.580222 11 179.877116 0
Cl 46 1.749821 44 119.586806 43 -179.918073 0
Cl 22 1.749821 20 119.586806 19 -179.918073 0
Cl 31 1.751771 26 116.633814 3 2.280919 0
Cl 30 1.752852 28 115.706920 27 -176.458499 0
Cl 7 1.752852 5 115.706920 4 -176.458499 0
Cl 35 1.753375 34 121.092191 33 -3.759172 0
Cl 11 1.753375 10 121.092191 9 -3.759172 0
Cl 43 1.754121 42 121.132939 33 -4.718598 0
Cl 19 1.754121 18 121.132939 9 -4.718598 0
Cl 49 1.754381 47 115.452125 46 -176.224378 0
Cl 25 1.754381 23 115.452125 22 -176.224378 0
Cl 41 1.755145 39 115.528237 38 -176.221696 0
Cl 17 1.755145 15 115.528237 14 -176.221696 0
```

**Geometry at $\theta = 110.000^{\mathbf{o}}$**

```
Cl
C  1 1.753122
C  2 1.404165 1 116.489222
C  3 1.403236 2 117.104344 1 -175.716474 0
C  4 1.389390 3 121.512421 2 1.784679 0
H  5 1.082136 4 120.249438 3 -179.142203 0
C  5 1.387828 4 119.558360 3 -1.191336 0
C  7 1.415679 5 122.665889 4 0.319790 0
C  8 1.476859 7 122.242202 5 179.593250 0
C  9 1.473868 8 120.133607 7 130.121698 0
C  10 1.418996 9 122.723367 8 -48.165459 0
C  11 1.390845 10 123.252193 9 179.312014 0
H  12 1.082391 11 120.149000 10 179.155858 0
C  12 1.390707 11 118.978846 10 0.388694 0
C  14 1.390514 12 120.857290 11 -0.012209 0
H  15 1.082153 14 120.918205 12 -178.875173 0
C  15 1.390599 14 118.948318 12 -0.251061 0
C  9 1.474321 8 119.676476 7 -49.645608 0
C  18 1.419454 9 122.639677 8 131.072841 0
C  19 1.390759 18 123.297409 9 -179.788923 0
H  20 1.082213 19 120.169105 18 178.889036 0
C  20 1.390576 19 118.913218 18 0.230435 0
C  22 1.390551 20 120.886379 19 -0.231310 0
H  23 1.082333 22 120.871921 20 -178.792700 0
C  23 1.390746 22 119.005728 20 -0.012640 0
C  3 1.492927 2 121.615188 1 9.333902 0
```

```
C  26 1.403236 3 121.083368 2 75.250015 0
C  27 1.389390 26 121.512421 3 176.762854 0
H  28 1.082136 27 120.249438 26 -179.142203 0
C  28 1.387828 27 119.558360 26 -1.191336 0
C  26 1.404165 3 121.615188 2 -110.000003 0
C  30 1.415679 28 122.665889 27 0.319790 0
C  32 1.476859 30 122.242202 28 179.593250 0
C  33 1.473868 32 120.133607 30 130.121698 0
C  34 1.418996 33 122.723367 32 -48.165459 0
C  35 1.390845 34 123.252193 33 179.312014 0
H  36 1.082391 35 120.149000 34 179.155858 0
C  36 1.390707 35 118.978846 34 0.388694 0
C  38 1.390514 36 120.857290 35 -0.012209 0
H  39 1.082153 38 120.918205 36 -178.875173 0
C  39 1.390599 38 118.948318 36 -0.251061 0
C  33 1.474321 32 119.676476 30 -49.645608 0
C  42 1.419454 33 122.639677 32 131.072841 0
C  43 1.390759 42 123.297409 33 -179.788923 0
H  44 1.082213 43 120.169105 42 178.889036 0
C  44 1.390576 43 118.913218 42 0.230435 0
C  46 1.390551 44 120.886379 43 -0.231310 0
H  47 1.082333 46 120.871921 44 -178.792700 0
C  47 1.390746 46 119.005728 44 -0.012640 0
Cl 27 1.748529 26 120.773911 3 -2.011653 0
Cl 4 1.748529 3 120.773911 2 -176.989828 0
Cl 38 1.749702 36 119.619410 35 -179.980240 0
Cl 14 1.749702 12 119.619410 11 -179.980240 0
Cl 46 1.749929 44 119.576230 43 179.661839 0
Cl 22 1.749929 20 119.576230 19 179.661839 0
Cl 30 1.753015 28 115.801830 27 -176.031475 0
Cl 7 1.753015 5 115.801830 4 -176.031475 0
Cl 31 1.753122 26 116.489222 3 9.333902 0
Cl 49 1.753650 47 115.512744 46 -176.314223 0
Cl 25 1.753650 23 115.512744 22 -176.314223 0
Cl 41 1.754523 39 115.457443 38 -176.239871 0
Cl 17 1.754523 15 115.457443 14 -176.239871 0
Cl 35 1.754574 34 121.126473 33 -4.386325 0
Cl 11 1.754574 10 121.126473 9 -4.386325 0
Cl 43 1.754663 42 121.133346 33 -3.557135 0
Cl 19 1.754663 18 121.133346 9 -3.557135 0
```

### S7.3 Removing two methyl substituents from the methylated benzylic radical *m*-dimer

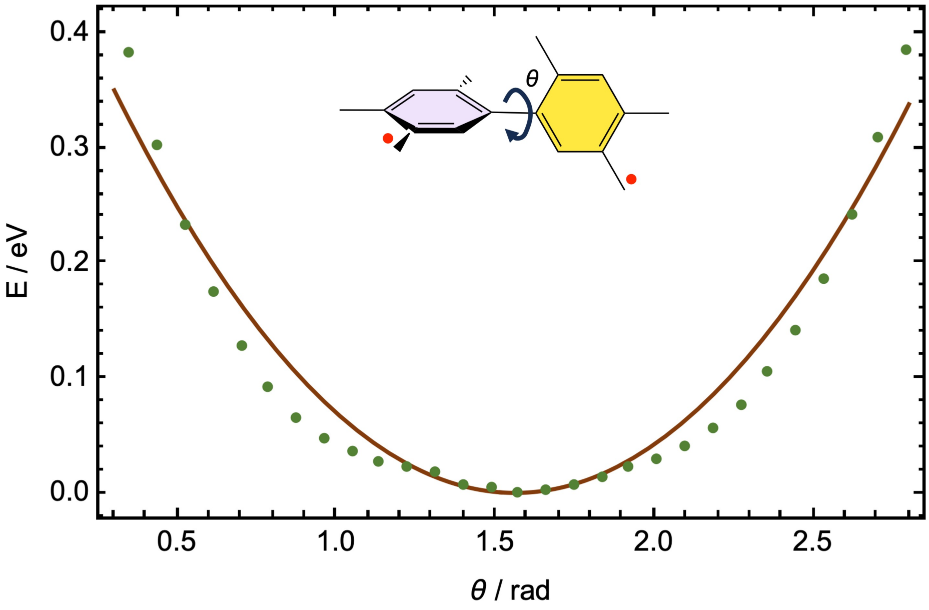


**FIG. S4**: Ground-state PES of the methylated benzylic radical *m*-dimer over different torsional angles $\theta$ after removing the *ortho*-methyl substituents facing the dimer linkage. (Green) Relative energies from a PES scan of the triplet configuration using DFT at the UB3LYP/6–31G(d,p) level. (Brown) Plot of $V_{\mathrm{steric}}(\theta) = E_{\mathrm{steric}}(\theta - \theta_{\mathrm{eq}})^2$ using the fitted parameters of $E_{\mathrm{steric}} = 0.220\,\mathrm{eV\,rad}^{-1}$ and $\theta_{\mathrm{eq}} = 1.561$ rad.

## S8 Results from ab initio calculations of AHRs

### S8.1 Methylated benzylic radical

The SCF calculation converged to an energy of -388.8867831125 Hartree and an $\langle \mathbf{S}^2 \rangle$ value of 0.784892232.

**Table S8**: Key electronic transitions of the methylated benzylic radical, calculated using TDDFT/TDA at the UB3LYP/6–31G(d,p) level.

| Energy / eV | $\langle \mathbf{S}^2 \rangle$ | Oscillator strength | Main contributions (sign) | Assignment |
|---|---|---|---|---|
| 3.0802 | 0.8435 | 0.0044487822 | $36\,\beta \to 37\,\beta\,(+)$<br>$37\,\alpha \to 38\,\alpha\,(+)$ | $\lvert\Psi^{-}_{01}; +1/2\rangle$ |
| 3.4101 | 0.8425 | 0.0103001979 | $35\,\beta \to 37\,\beta\,(+)$<br>$37\,\alpha \to 39\,\alpha\,(+)$ | $\lvert\Psi^{-}_{02}; +1/2\rangle$ |
| 4.0035 | 0.9006 | 0.0695851770 | $37\,\alpha \to 38\,\alpha\,(+)$<br>$36\,\beta \to 37\,\beta\,(-)$ | $\lvert\Psi^{+}_{01}; +1/2\rangle$ |
| 5.2016 | 0.8524 | 0.3740902854 | $37\,\alpha \to 39\,\alpha\,(+)$<br>$35\,\beta \to 37\,\beta\,(-)$ | $\lvert\Psi^{+}_{02}; +1/2\rangle$ |

## Optimised geometry

```
C
C  1 1.401417
H  2 1.082238 1 121.754082
H  2 1.082253 1 121.794892 3 -179.970652 0
C  1 1.440113 2 121.034980 3 0.057816 0
C  5 1.388984 1 119.661480 2 179.957364 0
H  6 1.088027 5 118.775280 1 -179.973799 0
C  6 1.402451 5 122.396270 1 -0.017491 0
C  8 1.406359 6 117.909635 5 -0.012993 0
H  9 1.088405 8 118.871406 6 -179.876368 0
C  9 1.385794 8 122.348414 6 0.038432 0
C  8 1.508017 6 121.341711 5 179.683170 0
H  12 1.093289 8 111.390407 6 3.192378 0
H  12 1.096604 8 111.479725 6 123.681384 0
H  12 1.097126 8 111.451286 6 -117.120122 0
C  5 1.508241 1 120.592261 2 -0.013536 0
H  16 1.092956 5 110.894195 1 179.882668 0
H  16 1.096787 5 111.723058 1 59.677967 0
H  16 1.096815 5 111.721412 1 -59.912630 0
C  11 1.508312 9 119.840576 8 179.993808 0
H  20 1.092964 11 110.898636 9 -0.550835 0
H  20 1.096669 11 111.706966 9 -120.765074 0
H  20 1.096810 11 111.701013 9 119.666405 0
```

## Orbital energies in Hartrees

```
 Alpha MOs
 -- Occupied --
-10.1926 -10.1923 -10.1920 -10.1866 -10.1811 -10.1807 -10.1785 -10.1784
-10.1749 -10.1746  -0.8559  -0.7867  -0.7770  -0.7169  -0.6953  -0.6726
 -0.6303  -0.5673  -0.5531  -0.4848  -0.4775  -0.4281  -0.4252  -0.4107
 -0.4087  -0.4048  -0.3986  -0.3971  -0.3921  -0.3780  -0.3587  -0.3346
 -0.3315  -0.3203  -0.2735  -0.2367  -0.1669
 -- Virtual --
  0.0093   0.0298   0.1008   0.1119   0.1209   0.1322   0.1392   0.1424
  0.1640   0.1738   0.1781   0.1824   0.1884   0.1894   0.2107   0.2129
  0.2454   0.2515   0.2645   0.3015   0.3514   0.3606   0.3716   0.3893
  0.4484   0.4844   0.5101   0.5157   0.5393   0.5440   0.5490   0.5634
  0.5753   0.5848   0.5901   0.5980   0.6144   0.6167   0.6582   0.6745
  0.6868   0.7135   0.7194   0.7264   0.7279   0.7414   0.7544   0.7675
  0.7839   0.8195   0.8257   0.8259   0.8349   0.8536   0.8659   0.8716
  0.8944   0.8993   0.9129   0.9287   0.9411   0.9533   0.9989   1.0087
  1.0160   1.0605   1.0933   1.1176   1.1416   1.1921   1.2050   1.2259
  1.2575   1.2705   1.3130   1.3157   1.3519   1.3662   1.3722   1.4102
  1.4197   1.4598   1.4745   1.5693   1.5845   1.7001   1.7197   1.7338
  1.7406   1.7612   1.7652   1.7912   1.8377   1.8427   1.8575   1.8591
  1.8811   1.8981   1.9610   1.9649   1.9732   1.9984   2.0141   2.0183
  2.0469   2.0487   2.0529   2.0872   2.0893   2.0935   2.1068   2.1380
  2.1535   2.1633   2.1838   2.1927   2.2070   2.2181   2.2192   2.2410
```

```
  2.3114   2.3279   2.3765   2.4115   2.4202   2.4428   2.4479   2.4607
  2.4772   2.5385   2.5421   2.5517   2.5587   2.5928   2.6322   2.6484
  2.6550   2.6667   2.6805   2.7276   2.7393   2.7924   2.7982   2.8477
  2.8541   2.8554   2.8644   2.8769   2.8778   2.8829   3.0369   3.0616
  3.0838   3.1822   3.1965   3.2073   3.2130   3.2572   3.3802   3.4151
  3.4279   3.4315   3.4326   3.4530   3.4727   3.4855   3.6146   3.7059
  4.1101   4.1486   4.1626   4.2530   4.3634   4.4123   4.4444   4.5645
  4.5835   4.8592

 Beta MOs
 -- Occupied --
-10.1894 -10.1890 -10.1886 -10.1880 -10.1810 -10.1788 -10.1787 -10.1766
-10.1763 -10.1720  -0.8517  -0.7806  -0.7733  -0.7080  -0.6950  -0.6738
 -0.6188  -0.5639  -0.5482  -0.4826  -0.4755  -0.4250  -0.4194  -0.4065
 -0.4057  -0.4024  -0.3974  -0.3957  -0.3901  -0.3755  -0.3581  -0.3293
 -0.3272  -0.3191  -0.2492  -0.2300
 -- Virtual --
 -0.0735   0.0195   0.0515   0.1017   0.1136   0.1217   0.1334   0.1425
  0.1467   0.1646   0.1762   0.1799   0.1847   0.1912   0.1937   0.2117
  0.2189   0.2490   0.2553   0.2678   0.3044   0.3529   0.3624   0.3730
  0.3904   0.4493   0.4863   0.5129   0.5190   0.5423   0.5463   0.5648
  0.5677   0.5772   0.5903   0.5921   0.6153   0.6181   0.6192   0.6702
  0.6751   0.6873   0.7167   0.7203   0.7282   0.7374   0.7435   0.7569
  0.7763   0.7872   0.8234   0.8254   0.8290   0.8342   0.8560   0.8684
  0.8734   0.8953   0.9022   0.9130   0.9302   0.9426   0.9547   1.0039
  1.0127   1.0215   1.0671   1.0952   1.1201   1.1443   1.1933   1.2070
  1.2286   1.2629   1.2760   1.3184   1.3200   1.3517   1.3696   1.3828
  1.4128   1.4257   1.4620   1.4988   1.5720   1.5884   1.7018   1.7214
  1.7384   1.7436   1.7621   1.7663   1.7933   1.8408   1.8473   1.8590
  1.8656   1.8974   1.8999   1.9645   1.9736   1.9789   2.0030   2.0135
  2.0223   2.0482   2.0499   2.0547   2.0898   2.0943   2.0954   2.1090
  2.1450   2.1556   2.1639   2.1914   2.2015   2.2067   2.2175   2.2221
  2.2457   2.3159   2.3306   2.3779   2.4127   2.4221   2.4446   2.4551
  2.4681   2.4785   2.5455   2.5474   2.5556   2.5704   2.5949   2.6353
  2.6545   2.6572   2.6739   2.6817   2.7293   2.7409   2.7935   2.7993
  2.8495   2.8551   2.8568   2.8659   2.8791   2.8798   2.8839   3.0398
  3.0627   3.0852   3.1834   3.1973   3.2086   3.2154   3.2588   3.3840
  3.4148   3.4295   3.4326   3.4339   3.4535   3.4731   3.4862   3.6190
  3.7063   4.1133   4.1528   4.1659   4.2681   4.3631   4.4151   4.4464
  4.5661   4.5866   4.8624
```

### Excited states from TDDFT/TDA

```
 Excited state   1: excitation energy (eV) =    3.0802
 Total energy for state  1:                   -388.77359883 au
    <S**2>     :  0.8435
    Trans. Mom.: -0.0022 X   0.2428 Y  -0.0001 Z
    Strength   :     0.0044487822
    S(    1) --> V(    1) amplitude =  0.4617 alpha
    D(   36) --> S(    1) amplitude =  0.8787 beta

 Excited state   2: excitation energy (eV) =    3.4101
```

```
Total energy for state  2:                    -388.76147426 au
   <S**2>     :  0.8425
   Trans. Mom.: -0.3473 X   0.0520 Y   0.0001 Z
   Strength   :     0.0103001979
   S(    1) --> V(    2) amplitude =  0.5888 alpha
   D(   35) --> S(    1) amplitude =  0.7901 beta

Excited state   3: excitation energy (eV) =    4.0035
Total energy for state  3:                    -388.73966630 au
   <S**2>     :  0.9006
   Trans. Mom.: -0.0926 X  -0.8372 Y   0.0005 Z
   Strength   :     0.0695851770
   S(    1) --> V(    1) amplitude =  0.8539 alpha
   D(   35) --> V(    1) amplitude =  0.1676 beta
   D(   36) --> S(    1) amplitude = -0.4395 beta

Excited state   4: excitation energy (eV) =    4.5314
Total energy for state  4:                    -388.72026636 au
   <S**2>     :  2.6575
   Trans. Mom.: -0.1837 X  -0.0051 Y   0.0004 Z
   Strength   :     0.0037511235
   D(   36) --> V(    1) amplitude =  0.7120 alpha
   D(   33) --> S(    1) amplitude =  0.1509 beta
   D(   36) --> V(    1) amplitude = -0.6463 beta

Excited state   5: excitation energy (eV) =    5.2016
Total energy for state  5:                    -388.69563862 au
   <S**2>     :  0.8524
   Trans. Mom.:  1.7132 X  -0.0171 Y  -0.0027 Z
   Strength   :     0.3740902854
   S(    1) --> V(    2) amplitude =  0.7467 alpha
   D(   35) --> S(    1) amplitude = -0.5379 beta
   D(   36) --> V(    1) amplitude = -0.2777 beta

Excited state   6: excitation energy (eV) =    5.3993
Total energy for state  6:                    -388.68837232 au
   <S**2>     :  0.8165
   Trans. Mom.: -0.0056 X  -0.0017 Y   0.0112 Z
   Strength   :     0.0000213317
   D(   34) --> S(    1) amplitude =  0.9893 beta
```

## S8.2 TTM

The SCF calculation converged to an energy of -4869.3523950252 Hartree and an $\langle \mathbf{S}^2 \rangle$ value of 0.770122243.

**Table S9**: Key electronic transitions of TTM, calculated using TDDFT/TDA at the UB3LYP/6–31G(d,p) level.

| Energy / eV | $\langle S^2 \rangle$ | Oscillator strength | Main contribution | Assignment |
|---|---|---|---|---|
| 2.7281 | 0.8880 | 0.0313358686 | $136\,\beta \rightarrow 137\,\beta$ | |
| 2.7285 | 0.8881 | 0.0309485674 | $135\,\beta \rightarrow 137\,\beta$ | |
| 2.9581 | 0.8504 | 0.0089904967 | $134\,\beta \rightarrow 137\,\beta$ | $\left\{\left\|\Psi^-_{0j}; +1/2\right\rangle \|1 \leq j \leq 5\right\}$ |
| 2.9622 | 0.8651 | 0.0077979747 | $133\,\beta \rightarrow 137\,\beta$ | |
| 2.9626 | 0.8655 | 0.0077560765 | $132\,\beta \rightarrow 137\,\beta$ | |
| 3.2083 | 0.9633 | 0.0000022116 | $131\,\beta \rightarrow 137\,\beta$ | $\left\|\Psi^-_{06}; +1/2\right\rangle$ |
| 3.4542 | 0.9972 | 0.2236567315 | $137\,\alpha \rightarrow 138\,\alpha$ | |
| 3.4586 | 0.9994 | 0.2251558495 | $137\,\alpha \rightarrow 139\,\alpha$ | |
| 3.6154 | 0.9600 | 0.0134795990 | $137\,\alpha \rightarrow 140\,\alpha$ | $\left\{\left\|\Psi^+_{0j}; +1/2\right\rangle \|1 \leq j \leq 5\right\}$ |
| 3.8078 | 1.0358 | 0.0025512786 | $137\,\alpha \rightarrow 141\,\alpha$ | |
| 3.8103 | 1.0372 | 0.0024961320 | $137\,\alpha \rightarrow 142\,\alpha$ | |

**Optimised geometry**

```
Cl
C  1 1.754165
C  2 1.390734 1 115.565389
H  3 1.082225 2 120.152346 1 -2.689353 0
C  3 1.390703 2 118.957480 1 176.161590 0
C  5 1.390687 3 120.892833 2 0.166266 0
H  6 1.082301 5 120.896230 3 178.792063 0
C  6 1.390814 5 118.929301 3 0.127814 0
C  8 1.419121 6 123.269660 5 -0.348016 0
C  9 1.474603 8 122.633894 6 -179.656507 0
C  10 1.474150 9 119.996029 8 49.113020 0
C  11 1.418896 10 122.674453 9 48.902969 0
C  12 1.390747 11 123.261458 10 -179.902948 0
H  13 1.082287 12 120.084967 11 -179.042116 0
C  13 1.390622 12 118.974203 11 -0.254731 0
C  15 1.390651 13 120.850369 12 0.039889 0
H  16 1.082310 15 120.926798 13 178.911948 0
C  16 1.390907 15 118.960721 13 0.235135 0
C  10 1.474505 9 119.943789 8 -131.186218 0
C  19 1.418865 10 122.632103 9 49.017468 0
C  20 1.390958 19 123.284184 10 -179.435463 0
H  21 1.082326 20 120.083080 19 -179.202059 0
C  21 1.390423 20 118.936828 19 -0.458268 0
C  23 1.390815 21 120.870440 20 0.062223 0
H  24 1.082316 23 120.856463 21 178.954611 0
C  24 1.390725 23 118.978413 21 0.248260 0
Cl 5 1.749706 3 119.526945 2 -179.992049 0
Cl 23 1.749780 21 119.546308 20 179.975256 0
Cl 15 1.749973 13 119.528692 12 179.885688 0
Cl 26 1.753908 24 115.539302 23 176.161861 0
```

```
Cl 8 1.754325 6 115.555971 5 176.182597 0
Cl 18 1.754437 16 115.516781 15 176.292285 0
Cl 12 1.754566 11 121.130407 10 3.892930 0
Cl 20 1.755086 19 121.131852 10 4.281575 0
```

## Orbital energies in Hartrees

```
 Alpha MOs
 -- Occupied --
********-101.5689-101.5688-101.5658-101.5657-101.5657-101.5657-101.5657
******** -10.2840 -10.2840 -10.2840 -10.2840 -10.2839 -10.2839 -10.2817
-10.2817 -10.2817 -10.2564 -10.2479 -10.2479 -10.2479 -10.2290 -10.2290
-10.2290 -10.2290 -10.2290 -10.2290  -9.4851  -9.4851  -9.4850  -9.4819
 -9.4819  -9.4819  -9.4818  -9.4818  -9.4818  -7.2492  -7.2491  -7.2489
 -7.2461  -7.2461  -7.2460  -7.2460  -7.2460  -7.2460  -7.2395  -7.2395
 -7.2394  -7.2389  -7.2389  -7.2389  -7.2362  -7.2361  -7.2361  -7.2361
 -7.2360  -7.2360  -7.2357  -7.2357  -7.2356  -7.2356  -7.2356  -7.2356
 -0.9456  -0.9314  -0.9314  -0.8984  -0.8916  -0.8916  -0.8915  -0.8882
 -0.8882  -0.8358  -0.8259  -0.8259  -0.8180  -0.7618  -0.7617  -0.7566
 -0.7563  -0.7562  -0.6899  -0.6339  -0.6338  -0.6274  -0.6232  -0.6231
 -0.5983  -0.5474  -0.5473  -0.5289  -0.5169  -0.5168  -0.5075  -0.4859
 -0.4859  -0.4762  -0.4617  -0.4616  -0.4567  -0.4567  -0.4563  -0.4391
 -0.4390  -0.4356  -0.4224  -0.4100  -0.4100  -0.4073  -0.3968  -0.3968
 -0.3865  -0.3840  -0.3839  -0.3781  -0.3728  -0.3728  -0.3407  -0.3367
 -0.3359  -0.3358  -0.3337  -0.3336  -0.3314  -0.3232  -0.3219  -0.3219
 -0.3148  -0.3148  -0.2962  -0.2680  -0.2680  -0.2670  -0.2615  -0.2615
 -0.2114
 -- Virtual --
 -0.0542  -0.0540  -0.0476  -0.0394  -0.0393  -0.0203  -0.0153  -0.0153
 -0.0035   0.0354   0.0373   0.0374   0.0392   0.0393   0.0397   0.1029
  0.1029   0.1295   0.1355   0.1375   0.1375   0.1498   0.1498   0.1568
  0.1802   0.2045   0.2047   0.2376   0.2377   0.2495   0.2501   0.2501
  0.2549   0.2659   0.2660   0.2675   0.2676   0.2751   0.3050   0.3051
  0.3120   0.3347   0.3348   0.3615   0.3615   0.3617   0.3701   0.3702
  0.3776   0.3810   0.3812   0.3833   0.3837   0.3837   0.3974   0.4011
  0.4012   0.4058   0.4164   0.4165   0.4166   0.4261   0.4262   0.4265
  0.4348   0.4364   0.4364   0.4428   0.4428   0.4562   0.4585   0.4591
  0.4592   0.4743   0.5053   0.5056   0.5165   0.5209   0.5212   0.5354
  0.5355   0.5508   0.5549   0.5559   0.5560   0.5677   0.5678   0.5720
  0.5735   0.5735   0.5797   0.5855   0.5928   0.5929   0.5988   0.5990
  0.6147   0.6284   0.6297   0.6354   0.6354   0.6438   0.6440   0.6714
  0.6715   0.6846   0.6957   0.6958   0.7079   0.7082   0.7148   0.7235
  0.7360   0.7360   0.7483   0.7485   0.7549   0.7549   0.7581   0.7760
  0.7929   0.8010   0.8011   0.8073   0.8140   0.8141   0.8204   0.8207
  0.8269   0.8418   0.8421   0.8456   0.8474   0.8485   0.8485   0.8535
  0.8536   0.8537   0.8659   0.8661   0.8692   0.8711   0.8894   0.8894
  0.8937   0.8995   0.8996   0.9036   0.9092   0.9093   0.9173   0.9259
  0.9261   0.9491   0.9492   0.9510   0.9566   0.9761   0.9764   0.9798
  0.9841   0.9843   1.0134   1.0137   1.0139   1.0199   1.0247   1.0250
  1.0494   1.0496   1.0543   1.0929   1.0930   1.0998   1.1117   1.1136
  1.1137   1.1189   1.1342   1.1344   1.1470   1.1488   1.1489   1.1502
  1.1806   1.1809   1.2050   1.2100   1.2105   1.2446   1.2752   1.2894
```

```
  1.2895   1.3015   1.3016   1.3469   1.3548   1.3549   1.3733   1.3734
  1.3772   1.3931   1.3972   1.3977   1.4261   1.4263   1.4264   1.4332
  1.4357   1.4358   1.4852   1.5202   1.5247   1.5253   1.5277   1.5277
  1.5465   1.5466   1.5698   1.5714   1.6057   1.6435   1.6440   1.7107
  1.7164   1.7166   1.7516   1.7517   1.7931   1.8091   1.8095   1.8101
  1.8306   1.8571   1.8572   1.8815   1.8816   1.8861   1.8921   1.9275
  1.9277   1.9391   1.9392   1.9995   2.0063   2.0064   2.0115   2.0141
  2.0141   2.0394   2.0496   2.0497   2.0677   2.0698   2.0718   2.0718
  2.1075   2.1077   2.1543   2.1544   2.1596   2.1779   2.2220   2.2221
  2.2420   2.2581   2.2584   2.2675   2.2680   2.2944   2.2944   2.4018
  2.4032   2.4034   2.4266   2.4268   2.4688   2.4896   2.4896   2.4967
  2.5276   2.5277   2.5490   2.5491   2.5677   2.5768   2.5798   2.5801
  2.5841   2.5926   2.5927   2.5965   2.5968   2.6052   2.6583   2.6762
  2.6764   2.7085   2.7261   2.7261   2.8316   2.8493   2.8494   2.8711
  2.9030   2.9062   2.9062   2.9724   2.9728   3.0982   3.1488   3.1519
  3.1521   3.1705   3.1707   3.3510   3.3526   3.3527   3.5651   3.5725
  3.5726   4.0501   4.0525   4.0526   4.0584   4.0589   4.0590   4.0859
  4.1107   4.1108   4.2300   4.2398   4.2400   4.2485   4.2716   4.2717
  4.3063   4.3064   4.3275   4.3616   4.3727   4.3731   4.4013   4.4287
  4.4289   4.4718   4.6889   4.6891   4.7339

 Beta MOs
 -- Occupied --
********-101.5688-101.5688-101.5658-101.5657-101.5657-101.5657-101.5657
******** -10.2824 -10.2824 -10.2824 -10.2824 -10.2824 -10.2824 -10.2804
-10.2804 -10.2804 -10.2495 -10.2494 -10.2494 -10.2456 -10.2296 -10.2296
-10.2296 -10.2296 -10.2296 -10.2295  -9.4850  -9.4850  -9.4850  -9.4819
 -9.4818  -9.4818  -9.4818  -9.4818  -9.4818  -7.2492  -7.2491  -7.2490
 -7.2461  -7.2461  -7.2461  -7.2461  -7.2461  -7.2461  -7.2392  -7.2392
 -7.2392  -7.2389  -7.2389  -7.2388  -7.2361  -7.2360  -7.2360  -7.2360
 -7.2359  -7.2359  -7.2356  -7.2356  -7.2356  -7.2356  -7.2356  -7.2356
 -0.9425  -0.9301  -0.9301  -0.8962  -0.8905  -0.8905  -0.8904  -0.8872
 -0.8871  -0.8303  -0.8256  -0.8256  -0.8135  -0.7615  -0.7614  -0.7566
 -0.7562  -0.7562  -0.6805  -0.6319  -0.6318  -0.6244  -0.6215  -0.6215
 -0.5948  -0.5461  -0.5460  -0.5242  -0.5161  -0.5161  -0.5053  -0.4847
 -0.4846  -0.4755  -0.4597  -0.4596  -0.4563  -0.4563  -0.4558  -0.4365
 -0.4364  -0.4317  -0.4211  -0.4086  -0.4086  -0.4044  -0.3956  -0.3955
 -0.3842  -0.3814  -0.3813  -0.3751  -0.3703  -0.3703  -0.3391  -0.3364
 -0.3357  -0.3357  -0.3336  -0.3335  -0.3299  -0.3224  -0.3218  -0.3218
 -0.3138  -0.3138  -0.2780  -0.2667  -0.2666  -0.2656  -0.2605  -0.2605
 -- Virtual --
 -0.1264  -0.0505  -0.0503  -0.0446  -0.0364  -0.0363  -0.0178  -0.0133
 -0.0132   0.0112   0.0373   0.0389   0.0390   0.0406   0.0406   0.0413
  0.1051   0.1052   0.1335   0.1360   0.1375   0.1375   0.1501   0.1502
  0.1584   0.1875   0.2065   0.2067   0.2391   0.2392   0.2501   0.2502
  0.2556   0.2564   0.2660   0.2661   0.2676   0.2755   0.2809   0.3071
  0.3072   0.3126   0.3351   0.3352   0.3623   0.3623   0.3632   0.3706
  0.3707   0.3796   0.3817   0.3820   0.3852   0.3852   0.3855   0.3980
  0.4026   0.4027   0.4062   0.4171   0.4171   0.4184   0.4267   0.4268
  0.4270   0.4358   0.4372   0.4372   0.4431   0.4432   0.4573   0.4594
  0.4597   0.4598   0.4822   0.5062   0.5065   0.5212   0.5215   0.5222
  0.5363   0.5364   0.5521   0.5561   0.5565   0.5566   0.5683   0.5685
  0.5734   0.5736   0.5736   0.5818   0.5842   0.5932   0.5933   0.6009
```

| | | | | | | | |
|---|---|---|---|---|---|---|---|
| 0.6012 | 0.6183 | 0.6306 | 0.6315 | 0.6363 | 0.6363 | 0.6458 | 0.6460 |
| 0.6732 | 0.6733 | 0.6873 | 0.6971 | 0.6972 | 0.7082 | 0.7084 | 0.7155 |
| 0.7320 | 0.7370 | 0.7370 | 0.7506 | 0.7507 | 0.7560 | 0.7561 | 0.7591 |
| 0.7826 | 0.7929 | 0.8009 | 0.8010 | 0.8077 | 0.8143 | 0.8144 | 0.8214 |
| 0.8217 | 0.8284 | 0.8424 | 0.8426 | 0.8468 | 0.8482 | 0.8492 | 0.8493 |
| 0.8541 | 0.8542 | 0.8544 | 0.8667 | 0.8669 | 0.8707 | 0.8717 | 0.8900 |
| 0.8901 | 0.8958 | 0.9004 | 0.9005 | 0.9052 | 0.9103 | 0.9104 | 0.9188 |
| 0.9266 | 0.9268 | 0.9499 | 0.9500 | 0.9561 | 0.9617 | 0.9773 | 0.9777 |
| 0.9804 | 0.9853 | 0.9855 | 1.0150 | 1.0152 | 1.0192 | 1.0219 | 1.0252 |
| 1.0255 | 1.0502 | 1.0503 | 1.0534 | 1.0941 | 1.0942 | 1.1039 | 1.1128 |
| 1.1148 | 1.1150 | 1.1220 | 1.1355 | 1.1356 | 1.1488 | 1.1501 | 1.1502 |
| 1.1506 | 1.1819 | 1.1821 | 1.2069 | 1.2111 | 1.2116 | 1.2483 | 1.2791 |
| 1.2913 | 1.2914 | 1.3020 | 1.3022 | 1.3483 | 1.3551 | 1.3551 | 1.3735 |
| 1.3737 | 1.3788 | 1.3940 | 1.3988 | 1.3993 | 1.4277 | 1.4280 | 1.4283 |
| 1.4342 | 1.4366 | 1.4368 | 1.4897 | 1.5220 | 1.5267 | 1.5274 | 1.5301 |
| 1.5302 | 1.5494 | 1.5494 | 1.5726 | 1.5736 | 1.6082 | 1.6479 | 1.6485 |
| 1.7111 | 1.7174 | 1.7175 | 1.7529 | 1.7531 | 1.8056 | 1.8109 | 1.8117 |
| 1.8120 | 1.8371 | 1.8611 | 1.8611 | 1.8838 | 1.8839 | 1.8861 | 1.8922 |
| 1.9366 | 1.9368 | 1.9438 | 1.9439 | 2.0020 | 2.0088 | 2.0088 | 2.0149 |
| 2.0173 | 2.0173 | 2.0416 | 2.0520 | 2.0521 | 2.0678 | 2.0722 | 2.0723 |
| 2.0736 | 2.1087 | 2.1089 | 2.1576 | 2.1577 | 2.1611 | 2.1773 | 2.2239 |
| 2.2240 | 2.2437 | 2.2610 | 2.2613 | 2.2694 | 2.2827 | 2.2976 | 2.2976 |
| 2.4031 | 2.4061 | 2.4063 | 2.4336 | 2.4338 | 2.4806 | 2.4891 | 2.4892 |
| 2.5056 | 2.5284 | 2.5285 | 2.5497 | 2.5499 | 2.5674 | 2.5772 | 2.5808 |
| 2.5811 | 2.5845 | 2.5936 | 2.5937 | 2.5981 | 2.5984 | 2.6090 | 2.6590 |
| 2.6769 | 2.6770 | 2.7101 | 2.7290 | 2.7291 | 2.8371 | 2.8507 | 2.8508 |
| 2.8720 | 2.9036 | 2.9070 | 2.9070 | 2.9744 | 2.9748 | 3.0988 | 3.1497 |
| 3.1538 | 3.1540 | 3.1715 | 3.1716 | 3.3509 | 3.3526 | 3.3527 | 3.5653 |
| 3.5727 | 3.5727 | 4.0526 | 4.0543 | 4.0544 | 4.0601 | 4.0604 | 4.0605 |
| 4.0875 | 4.1125 | 4.1126 | 4.2330 | 4.2394 | 4.2395 | 4.2482 | 4.2716 |
| 4.2717 | 4.3064 | 4.3066 | 4.3313 | 4.3648 | 4.3734 | 4.3738 | 4.4022 |
| 4.4283 | 4.4285 | 4.4817 | 4.6892 | 4.6894 | 4.7384 | | |

### Excited states from TDDFT/TDA

```
Excited state   1: excitation energy (eV) =    2.7281
Total energy for state  1:                 -4869.25209542 au
   <S**2>     :  0.8880
   Trans. Mom.: -0.6714 X   0.1344 Y   0.0007 Z
   Strength   :     0.0313358686
   S(    1) --> V(    2) amplitude =  0.2669 alpha
   D(  133) --> S(    1) amplitude = -0.1747 beta
   D(  136) --> S(    1) amplitude =  0.9191 beta

Excited state   2: excitation energy (eV) =    2.7285
Total energy for state  2:                 -4869.25208239 au
   <S**2>     :  0.8881
   Trans. Mom.: -0.1337 X  -0.6672 Y   0.0007 Z
   Strength   :     0.0309485674
   S(    1) --> V(    1) amplitude =  0.2678 alpha
   D(  132) --> S(    1) amplitude = -0.1745 beta
   D(  135) --> S(    1) amplitude =  0.9188 beta
```

```
Excited state   3: excitation energy (eV) =    2.9581
Total energy for state  3:                 -4869.24364404 au
   <S**2>     :  0.8504
   Trans. Mom.:  0.0534 X  -0.0076 Y   0.3481 Z
   Strength   :     0.0089904967
   S(    1) --> V(    3) amplitude =  0.1703 alpha
   D(  134) --> S(    1) amplitude =  0.9607 beta

Excited state   4: excitation energy (eV) =    2.9622
Total energy for state  4:                 -4869.24349239 au
   <S**2>     :  0.8651
   Trans. Mom.:  0.2421 X  -0.2160 Y  -0.0469 Z
   Strength   :     0.0077979747
   S(    1) --> V(    2) amplitude = -0.1661 alpha
   D(  132) --> S(    1) amplitude = -0.1961 beta
   D(  133) --> S(    1) amplitude =  0.8961 beta
   D(  136) --> S(    1) amplitude =  0.1997 beta

Excited state   5: excitation energy (eV) =    2.9626
Total energy for state  5:                 -4869.24348018 au
   <S**2>     :  0.8655
   Trans. Mom.:  0.2156 X   0.2439 Y  -0.0294 Z
   Strength   :     0.0077560765
   S(    1) --> V(    1) amplitude = -0.1698 alpha
   D(  132) --> S(    1) amplitude =  0.9018 beta
   D(  133) --> S(    1) amplitude =  0.1878 beta
   D(  135) --> S(    1) amplitude =  0.2031 beta

Excited state   6: excitation energy (eV) =    3.2083
Total energy for state  6:                 -4869.23444938 au
   <S**2>     :  0.9633
   Trans. Mom.: -0.0002 X  -0.0049 Y   0.0019 Z
   Strength   :     0.0000022116
   S(    1) --> V(    9) amplitude = -0.2535 alpha
   D(  131) --> S(    1) amplitude =  0.9118 beta

Excited state   7: excitation energy (eV) =    3.4542
Total energy for state  7:                 -4869.22541154 au
   <S**2>     :  0.9972
   Trans. Mom.:  0.2293 X   1.6094 Y  -0.0018 Z
   Strength   :     0.2236567315
   S(    1) --> V(    1) amplitude =  0.8772 alpha
   D(  132) --> S(    1) amplitude =  0.2496 beta
   D(  135) --> S(    1) amplitude = -0.2399 beta

Excited state   8: excitation energy (eV) =    3.4586
Total energy for state  8:                 -4869.22525163 au
   <S**2>     :  0.9994
   Trans. Mom.:  1.6137 X  -0.2305 Y   0.0041 Z
   Strength   :     0.2251558495
   S(    1) --> V(    2) amplitude =  0.8770 alpha
   D(  133) --> S(    1) amplitude =  0.2485 beta
```

```
   D(  136) --> S(    1) amplitude = -0.2393 beta

Excited state   9: excitation energy (eV) =    3.6154
Total energy for state  9:                 -4869.21948916 au
   <S**2>     :  0.9600
   Trans. Mom.:  0.0072 X  -0.0073 Y  -0.3900 Z
   Strength   :     0.0134795990
   S(    1) --> V(    3) amplitude =  0.9529 alpha
   D(  134) --> S(    1) amplitude = -0.1777 beta

Excited state  10: excitation energy (eV) =    3.8078
Total energy for state 10:                 -4869.21241806 au
   <S**2>     :  1.0358
   Trans. Mom.: -0.0566 X  -0.1554 Y   0.0021 Z
   Strength   :     0.0025512786
   S(    1) --> V(    4) amplitude =  0.9382 alpha

Excited state  11: excitation energy (eV) =    3.8103
Total energy for state 11:                 -4869.21232661 au
   <S**2>     :  1.0372
   Trans. Mom.: -0.1542 X   0.0543 Y  -0.0018 Z
   Strength   :     0.0024961320
   S(    1) --> V(    5) amplitude =  0.9378 alpha

Excited state  12: excitation energy (eV) =    3.9515
Total energy for state 12:                 -4869.20713792 au
   <S**2>     :  2.5780
   Trans. Mom.:  0.0002 X  -0.0007 Y  -0.0002 Z
   Strength   :     0.0000000596
   D(  132) --> V(    1) amplitude =  0.1630 alpha
   D(  132) --> V(    4) amplitude = -0.2163 alpha
   D(  133) --> V(    2) amplitude =  0.1625 alpha
   D(  133) --> V(    5) amplitude = -0.2157 alpha
   D(  134) --> V(    3) amplitude = -0.3314 alpha
   D(  135) --> V(    1) amplitude = -0.1913 alpha
   D(  135) --> V(    4) amplitude = -0.1854 alpha
   D(  136) --> V(    2) amplitude = -0.1884 alpha
   D(  136) --> V(    5) amplitude = -0.1863 alpha
   D(  131) --> S(    1) amplitude = -0.2687 beta
   D(  132) --> V(    1) amplitude =  0.1736 beta
   D(  132) --> V(    4) amplitude = -0.2004 beta
   D(  133) --> V(    2) amplitude = -0.1731 beta
   D(  133) --> V(    5) amplitude = -0.2000 beta
   D(  134) --> V(    3) amplitude = -0.3009 beta
   D(  135) --> V(    1) amplitude = -0.2429 beta
   D(  135) --> V(    4) amplitude = -0.1688 beta
   D(  136) --> V(    2) amplitude =  0.2405 beta
   D(  136) --> V(    5) amplitude = -0.1695 beta

Excited state  13: excitation energy (eV) =    4.0679
Total energy for state 13:                 -4869.20285902 au
   <S**2>     :  2.5489
   Trans. Mom.:  0.0324 X  -0.1957 Y  -0.0003 Z
```

```
   Strength   :     0.0039214477
   D(  132) --> V(    3) amplitude =  0.2029 alpha
   D(  132) --> V(    4) amplitude =  0.1957 alpha
   D(  133) --> V(    3) amplitude =  0.2318 alpha
   D(  133) --> V(    5) amplitude = -0.1948 alpha
   D(  134) --> V(    5) amplitude =  0.2945 alpha
   D(  135) --> V(    1) amplitude = -0.1608 alpha
   D(  136) --> V(    2) amplitude =  0.1574 alpha
   D(  136) --> V(    3) amplitude =  0.2296 alpha
   S(    1) --> V(    1) amplitude = -0.2323 alpha
   D(  132) --> V(    3) amplitude =  0.1982 beta
   D(  132) --> V(    4) amplitude =  0.1950 beta
   D(  133) --> V(    3) amplitude =  0.2424 beta
   D(  133) --> V(    5) amplitude = -0.1954 beta
   D(  134) --> V(    5) amplitude =  0.2915 beta
   D(  136) --> V(    3) amplitude =  0.2128 beta

Excited state  14: excitation energy (eV) =    4.0684
Total energy for state 14:                 -4869.20284124 au
   <S**2>     :  2.5477
   Trans. Mom.: -0.1983 X  -0.0317 Y   0.0002 Z
   Strength   :     0.0040192136
   D(  132) --> V(    3) amplitude = -0.2315 alpha
   D(  132) --> V(    5) amplitude = -0.1953 alpha
   D(  133) --> V(    3) amplitude =  0.2009 alpha
   D(  133) --> V(    4) amplitude = -0.1945 alpha
   D(  134) --> V(    4) amplitude = -0.2957 alpha
   D(  135) --> V(    2) amplitude =  0.1601 alpha
   D(  135) --> V(    3) amplitude = -0.2254 alpha
   D(  136) --> V(    1) amplitude =  0.1607 alpha
   S(    1) --> V(    2) amplitude = -0.2333 alpha
   D(  132) --> V(    3) amplitude = -0.2413 beta
   D(  132) --> V(    5) amplitude = -0.1952 beta
   D(  133) --> V(    3) amplitude =  0.1963 beta
   D(  133) --> V(    4) amplitude = -0.1929 beta
   D(  134) --> V(    4) amplitude = -0.2946 beta
   D(  135) --> V(    3) amplitude = -0.2090 beta

Excited state  15: excitation energy (eV) =    4.3434
Total energy for state 15:                 -4869.19273364 au
   <S**2>     :  1.2222
   Trans. Mom.:  0.0253 X  -0.4519 Y   0.0037 Z
   Strength   :     0.0217967318
   D(  135) --> V(    1) amplitude = -0.1905 alpha
   D(  136) --> V(    2) amplitude =  0.1568 alpha
   S(    1) --> V(    8) amplitude =  0.2768 alpha
   D(  130) --> S(    1) amplitude =  0.7951 beta

Excited state  16: excitation energy (eV) =    4.3442
Total energy for state 16:                 -4869.19270713 au
   <S**2>     :  1.2169
   Trans. Mom.:  0.4578 X   0.0246 Y   0.0044 Z
   Strength   :     0.0223740371
```

```
D(  135) --> V(    2) amplitude = -0.1696 alpha
D(  136) --> V(    1) amplitude = -0.1774 alpha
S(    1) --> V(    7) amplitude = -0.2792 alpha
D(  129) --> S(    1) amplitude =  0.7954 beta
```

## References


[1] R. Pariser, The Journal of Chemical Physics **24**, 250 (1956).

[2] T. J. H. Hele, in *Physical Chemistry of Semiconductor Materials and Interfaces XX*, Vol. 11799, edited by A. J. Musser and D. Baran, International Society for Optics and Photonics (SPIE, 2021) p. 117991A.

[3] A. Szabo and N. S. Ostlund, *Modern Quantum Chemistry: Introduction to Advanced Electronic Structure Theory* (Dover Publications, 1989).

[4] W. Barford, R. J. Bursill, and D. V. Makhov, Physical Review B **81**, 035206 (2010).

[5] R. Englman and J. Jortner, Molecular Physics **18**, 145 (1970).

[6] Z. G. Yu, Physical Review B **85**, 115201 (2012).
